# Supplementary material for: Polishing the Gold Standard: The Role of Orbital Choice in CCSD(T) Vibrational Frequency Prediction
Source: arXiv:2007.08435 source file (2020-07-17)
Supplement: Supplementary file 1 [file ccsdt_frequencies_SI.pdf]

# Supporting Information: Polishing the gold standard: The role of orbital choice in CCSD(T) frequency prediction

Luke W. Bertels,† Joonho Lee,†,‡ and Martin Head-Gordon*,†,¶

†*Department of Chemistry, University of California, Berkeley, California 94720, USA.*

‡*Department of Chemistry, Columbia University, New York, New York 10027, USA.*

¶*Chemical Sciences Division, Lawrence Berkeley National Laboratory, Berkeley, California 94720, USA.*

E-mail: mhg@cchem.berkeley.edu

# Contents

**1 Equilibrium bond lengths** **S-2**

**2 Species not included in the test set** **S-14**

**3 Mean-field $\langle S^2 \rangle$ values** **S-14**

**4 CCSD data** **S-21**

# 1 Equilibrium bond lengths

Table S1: Root mean square deviations, mean signed deviations, most negative deviation, and most positive deviations in the equilibrium bond lengths for all species are are presented for the CCSD(T) methods utilizing different molecular orbital references.

| | Δ(CCSD(T): UHF) | Δ(CCSD(T): κ-OOMP2) | Δ(CCSD(T): OOMP2) | Δ(CCSD(T): BLYP) | Δ(CCSD(T): B97M-rV) | Δ(CCSD(T): B97) | Δ(CCSD(T): ωB97X-V) | Δ(CCSD(T): ωB97M-V) |
|---|---|---|---|---|---|---|---|---|
| RMSD | 0.02258 | 0.01283 | 0.01772 | 0.01338 | 0.01328 | 0.01330 | 0.01328 | 0.01331 |
| MSD | 0.00676 | 0.00627 | 0.00468 | 0.00639 | 0.00617 | 0.00616 | 0.00604 | 0.00611 |
| MIN | -0.01283 | -0.01153 | -0.08190 | -0.02182 | -0.02153 | -0.02277 | -0.02355 | -0.02448 |
| MAX | 0.17325 | 0.08127 | 0.08457 | 0.08479 | 0.08477 | 0.08473 | 0.08472 | 0.08471 |

Table S2: Experimental equilibrium bond lengths (in Å) and errors in the computed bond lengths (in Å) for the closed-shell species are presented for the CCSD(T) methods utilizing different molecular orbitals. Root mean square deviations, mean signed deviations, most negative deviations, and most positive deviations (all in Å) for the set of species and subsets are presented. Experimental values were compiled by Huber and Herzberg.[?]

| Row 2–Row 2 | Dimer | State | Expt. | Δ(CCSD(T): UHF) | Δ(CCSD(T): κ-OOMP2) | Δ(CCSD(T): OOMP2) | Δ(CCSD(T): BLYP) | Δ(CCSD(T): B97M-rV) | Δ(CCSD(T): B97) | Δ(CCSD(T): ωB97X-V) | Δ(CCSD(T): ωB97M-V) |
|---|---|---|---|---|---|---|---|---|---|---|---|
| | LiH | $X^1\Sigma^+$ | 1.5957 | 0.00180 | 0.00181 | 0.00181 | 0.00182 | 0.00182 | 0.00182 | 0.00181 | 0.00181 |
| | $Li_2$ | $X^1\Sigma_g^+$ | 2.6729 | 0.00462 | 0.00463 | 0.00463 | 0.00465 | 0.00466 | 0.00463 | 0.00462 | 0.00462 |
| | LiF | $X^1\Sigma^+$ | 1.56386 | 0.00439 | 0.00462 | 0.00477 | 0.00511 | 0.00480 | 0.00478 | 0.00472 | 0.00476 |
| | $BeH^+$ | $X^1\Sigma^+$ | 1.3122 | 0.00028 | 0.00028 | 0.00028 | 0.00029 | 0.00029 | 0.00029 | 0.00029 | 0.00029 |
| | BeO | $X^1\Sigma^+$ | 1.3309 | 0.00544 | 0.00556 | 0.00735 | 0.00676 | 0.00591 | 0.00598 | 0.00546 | 0.00560 |
| | BH | $X^1\Sigma^+$ | 1.2324 | -0.00038 | -0.00047 | -0.00080 | -0.00065 | -0.00075 | -0.00081 | -0.00082 | -0.00081 |
| | BF | $X^1\Sigma^+$ | 1.26259 | 0.00606 | 0.00642 | 0.00654 | 0.00687 | 0.00654 | 0.00658 | 0.00649 | 0.00651 |
| | $C_2$ | $X^1\Sigma_g^+$ | 1.24253 | -0.00631 | 0.00372 | 0.00464 | -0.02182 | -0.02153 | -0.02277 | -0.02355 | -0.02448 |
| | CO | $X^1\Sigma^+$ | 1.12832 | 0.00411 | 0.00429 | 0.00432 | 0.00445 | 0.00430 | 0.00433 | 0.00428 | 0.00428 |
| | $N_2$ | $X^1\Sigma_g^+$ | 1.09769 | 0.00260 | 0.00268 | 0.00268 | 0.00275 | 0.00267 | 0.00270 | 0.00267 | 0.00268 |
| | $NO^+$ | $X^1\Sigma^+$ | 1.06322 | 0.00245 | 0.00258 | 0.00257 | 0.00270 | 0.00258 | 0.00261 | 0.00258 | 0.00258 |
| | $OH^-$ | $X^1\Sigma^+$ | 0.97 | -0.00330 | -0.00322 | -0.00310 | -0.00321 | -0.00326 | -0.00325 | -0.00327 | -0.00327 |
| | HF | $X^1\Sigma^+$ | 0.91681 | 0.00349 | 0.00355 | 0.00356 | 0.00356 | 0.00351 | 0.00352 | 0.00352 | 0.00352 |
| | $F_2$ | $X^1\Sigma_g^+$ | 1.41193 | -0.01148 | 0.00452 | 0.00446 | 0.00447 | 0.00449 | 0.00452 | 0.00454 | 0.00456 |
| | RMSD | | | 0.00489 | 0.00385 | 0.00415 | 0.00706 | 0.00689 | 0.00718 | 0.00732 | 0.00755 |
| | MSD | | | 0.00098 | 0.00293 | 0.00312 | 0.00127 | 0.00115 | 0.00107 | 0.00095 | 0.00090 |
| | MIN | | | -0.01148 | -0.00322 | -0.00310 | -0.02182 | -0.02153 | -0.02277 | -0.02355 | -0.02448 |
| | MAX | | | 0.00606 | 0.00642 | 0.00735 | 0.00687 | 0.00654 | 0.00658 | 0.00649 | 0.00651 |
| Row 2–Row 3 | Dimer | State | Expt. | Δ(CCSD(T): UHF) | Δ(CCSD(T): κ-OOMP2) | Δ(CCSD(T): OOMP2) | Δ(CCSD(T): BLYP) | Δ(CCSD(T): B97M-rV) | Δ(CCSD(T): B97) | Δ(CCSD(T): ωB97X-V) | Δ(CCSD(T): ωB97M-V) |
| | NaH | $X^1\Sigma^+$ | 1.8874 | 0.00481 | 0.00481 | 0.00479 | 0.00498 | 0.00483 | 0.00490 | 0.00493 | 0.00487 |
| | NaLi | $X^1\Sigma^+$ | 2.81 | 0.08249 | 0.08127 | 0.08457 | 0.08479 | 0.08477 | 0.08473 | 0.08472 | 0.08471 |
| | NaF | $X^1\Sigma^+$ | 1.92595 | 0.00882 | 0.00904 | 0.00926 | 0.00968 | 0.00936 | 0.00930 | 0.00918 | 0.00919 |
| | $MgH^+$ | $X^1\Sigma^+$ | 1.6519 | 0.00387 | 0.00387 | 0.00384 | 0.00415 | 0.00386 | 0.00402 | 0.00400 | 0.00389 |
| | AlH | $X^1\Sigma^+$ | 1.6478 | 0.00092 | 0.00039 | 0.00039 | 0.00043 | 0.00046 | 0.00041 | 0.00039 | 0.00040 |
| | AlF | $X^1\Sigma^+$ | 1.65437 | 0.00577 | 0.00607 | 0.00623 | 0.00663 | 0.00625 | 0.00629 | 0.00617 | 0.00620 |
| | $SiH^+$ | $X^1\Sigma^+$ | 1.5041 | -0.00065 | -0.00089 | -0.00089 | -0.00085 | -0.00083 | -0.00086 | -0.00087 | -0.00086 |
| | SiO | $X^1\Sigma^+$ | 1.50974 | 0.00527 | 0.00548 | 0.00600 | 0.00597 | 0.00563 | 0.00563 | 0.00541 | 0.00541 |
| | PN | $X^1\Sigma^+$ | 1.49087 | -0.00451 | 0.00504 | 0.00523 | 0.00515 | 0.00496 | 0.00502 | 0.00497 | 0.00499 |
| | BeS | $X^1\Sigma^+$ | 1.74153 | 0.17325 | 0.00814 | 0.00821 | 0.00832 | 0.00821 | 0.00815 | 0.00812 | 0.00800 |
| | CS | $X^1\Sigma^+$ | 1.53494 | 0.00444 | 0.00471 | 0.00495 | 0.00504 | 0.00479 | 0.00481 | 0.00465 | 0.00468 |
| | $NS^+$ | $X^1\Sigma^+$ | 1.44 | -0.00806 | 0.00120 | 0.00125 | 0.00135 | 0.00117 | 0.00125 | 0.00119 | 0.00122 |

| | | | | | | | | | | |
|---|---|---|---|---|---|---|---|---|---|---|
| | HCl | $X^1\Sigma^+$ | 1.27455 | -0.00054 | -0.00053 | -0.00052 | -0.00054 | -0.00053 | -0.00053 | -0.00054 | -0.00053 |
| | LiCl | $X^1\Sigma^+$ | 2.02067 | 0.00775 | 0.00777 | 0.00779 | 0.00790 | 0.00784 | 0.00782 | 0.00778 | 0.00780 |
| | BCl | $X^1\Sigma^+$ | 1.7159 | 0.00408 | 0.00429 | 0.00460 | 0.00511 | 0.00479 | 0.00470 | 0.00436 | 0.00445 |
| | ClF | $X^1\Sigma^+$ | 1.62831 | 0.00677 | 0.00682 | 0.00686 | 0.00662 | 0.00647 | 0.00653 | 0.00658 | 0.00660 |
| | RMSD | | | 0.04824 | 0.02097 | 0.02180 | 0.02188 | 0.02183 | 0.02182 | 0.02180 | 0.02180 |
| | MSD | | | 0.01841 | 0.00922 | 0.00954 | 0.00967 | 0.00950 | 0.00951 | 0.00944 | 0.00944 |
| | MIN | | | -0.00806 | -0.00089 | -0.00089 | -0.00085 | -0.00083 | -0.00086 | -0.00087 | -0.00086 |
| | MAX | | | 0.17325 | 0.08127 | 0.08457 | 0.08479 | 0.08477 | 0.08473 | 0.08472 | 0.08471 |
| Row 3–Row 3 | Dimer | State | Expt. | Δ(CCSD(T): UHF) | Δ(CCSD(T): $\kappa$-OOMP2) | Δ(CCSD(T): OOMP2) | Δ(CCSD(T): BLYP) | Δ(CCSD(T): B97M-rV) | Δ(CCSD(T): B97) | Δ(CCSD(T): $\omega$B97X-V) | Δ(CCSD(T): $\omega$B97M-V) |
| | NaCl | $X^1\Sigma^+$ | 2.36079 | 0.01382 | 0.01381 | 0.01382 | 0.01392 | 0.01389 | 0.01387 | 0.01386 | 0.01382 |
| | AlCl | $X^1\Sigma^+$ | 2.13011 | 0.01496 | 0.01491 | 0.01508 | 0.01540 | 0.01521 | 0.01520 | 0.01504 | 0.01505 |
| | SiS | $X^1\Sigma^+$ | 1.92932 | 0.01042 | 0.01031 | 0.01057 | 0.01076 | 0.01053 | 0.01051 | 0.01031 | 0.01033 |
| | $P_2$ | $X^1\Sigma_g^+$ | 1.8934 | -0.00649 | 0.00874 | 0.00880 | 0.00882 | 0.00871 | 0.00874 | 0.00873 | 0.00874 |
| | $Cl_2$ | $X^1\Sigma_g^+$ | 1.9879 | 0.01591 | 0.01583 | 0.01586 | 0.01578 | 0.01578 | 0.01575 | 0.01582 | 0.01582 |
| | RMSD | | | 0.01280 | 0.01301 | 0.01311 | 0.01322 | 0.01312 | 0.01310 | 0.01305 | 0.01305 |
| | MSD | | | 0.00972 | 0.01272 | 0.01283 | 0.01294 | 0.01282 | 0.01281 | 0.01275 | 0.01275 |
| | MIN | | | -0.00649 | 0.00874 | 0.00880 | 0.00882 | 0.00871 | 0.00874 | 0.00873 | 0.00874 |
| | MAX | | | 0.01591 | 0.01583 | 0.01586 | 0.01578 | 0.01578 | 0.01575 | 0.01582 | 0.01582 |
| Closed-shell | Dimer | State | Expt. | Δ(CCSD(T): UHF) | Δ(CCSD(T): $\kappa$-OOMP2) | Δ(CCSD(T): OOMP2) | Δ(CCSD(T): BLYP) | Δ(CCSD(T): B97M-rV) | Δ(CCSD(T): B97) | Δ(CCSD(T): $\omega$B97X-V) | Δ(CCSD(T): $\omega$B97M-V) |
| | RMSD | | | 0.03311 | 0.01520 | 0.01577 | 0.01624 | 0.01617 | 0.01621 | 0.01622 | 0.01626 |
| | MSD | | | 0.01020 | 0.00720 | 0.00744 | 0.00678 | 0.00663 | 0.00660 | 0.00652 | 0.00650 |
| | MIN | | | -0.01148 | -0.00322 | -0.00310 | -0.02182 | -0.02153 | -0.02277 | -0.02355 | -0.02448 |
| | MAX | | | 0.17325 | 0.08127 | 0.08457 | 0.08479 | 0.08477 | 0.08473 | 0.08472 | 0.08471 |

Table S3: Experimental equilibrium bond lengths (in Å) and errors in the computed bond lengths (in Å) for the open-shell species are presented for the CCSD(T) methods utilizing different molecular orbitals. Root mean square deviations, mean signed deviations, most negative deviations, and most positive deviations (all in Å) for the set of species and subsets are presented. Experimental values were compiled by Huber and Herzberg.[?]

| Closed-shell | Dimer | State | Expt. | Δ(CCSD(T): UHF) | Δ(CCSD(T): κ-OOMP2) | Δ(CCSD(T): OOMP2) | Δ(CCSD(T): BLYP) | Δ(CCSD(T): B97M-rV) | Δ(CCSD(T): B97) | Δ(CCSD(T): ωB97X-V) | Δ(CCSD(T): ωB97M-V) |
|---|---|---|---|---|---|---|---|---|---|---|---|
| | LiO | $X^2\Pi_i$ | 1.695 | -0.00222 | -0.00218 | -0.00209 | -0.00173 | -0.00199 | -0.00203 | -0.00211 | -0.00207 |
| | BeH | $X^2\Sigma^+$ | 1.3426 | 0.00043 | 0.00043 | 0.00043 | 0.00047 | 0.00055 | 0.00046 | 0.00044 | 0.00048 |
| | BeF | $X^2\Sigma^+$ | 1.361 | 0.00378 | 0.00393 | 0.00400 | 0.00425 | 0.00404 | 0.00405 | 0.00399 | 0.00404 |
| | $B_2$ | $X^3\Sigma_g^-$ | 1.59 | -0.00741 | -0.00463 | 0.00106 | 0.00905 | 0.00398 | 0.00280 | -0.00081 | 0.00335 |
| | BN | $X^3\Pi$ | 1.281 | 0.04824 | 0.04909 | 0.04915 | 0.04917 | 0.04909 | 0.04908 | 0.04912 | 0.04914 |
| | BO | $X^2\Sigma^+$ | 1.2045 | 0.00498 | 0.00561 | 0.00580 | 0.00600 | 0.00573 | 0.00586 | 0.00571 | 0.00571 |
| | CH | $X^2\Pi_r$ | 1.1199 | 0.00095 | 0.00016 | 0.00016 | 0.00015 | 0.00017 | 0.00015 | 0.00015 | 0.00016 |
| | $C_2^-$ | $X^2\Sigma_g^+$ | 1.26821 | 0.04244 | 0.00393 | 0.00407 | 0.00407 | 0.00389 | 0.00394 | 0.00390 | 0.00591 |
| | CN | $X^2\Sigma^+$ | 1.17182 | -0.00157 | 0.00328 | 0.00340 | 0.00338 | 0.00321 | 0.00324 | 0.00322 | 0.00325 |
| | $CO^+$ | $X^2\Sigma^+$ | 1.11522 | 0.00023 | 0.00412 | 0.00441 | 0.00448 | 0.00399 | 0.00419 | 0.00413 | 0.00409 |
| | CF | $X^2\Pi_r$ | 1.2718 | 0.00518 | 0.00577 | 0.00598 | 0.00636 | 0.00588 | 0.00591 | 0.00578 | 0.00580 |
| | NH | $X^3\Sigma^-$ | 1.03621 | 0.00182 | 0.00181 | 0.00181 | 0.00180 | 0.00180 | 0.00181 | 0.00180 | 0.00180 |
| | $N_2^+$ | $X^2\Sigma_g^+$ | 1.11642 | -0.00207 | 0.00252 | 0.00254 | 0.00263 | 0.00248 | 0.00254 | 0.00249 | 0.00251 |
| | NO | $X^2\Pi_r$ | 1.15077 | -0.00019 | 0.00288 | 0.00285 | 0.00298 | 0.00289 | 0.00291 | 0.00289 | 0.00289 |
| | NF | $X^3\Sigma^-$ | 1.31698 | 0.00503 | 0.00572 | 0.00605 | 0.00644 | 0.00566 | 0.00576 | 0.00566 | 0.00563 |
| | OH | $X^2\Pi_i$ | 0.96966 | 0.00247 | 0.00247 | 0.00247 | 0.00246 | 0.00245 | 0.00246 | 0.00246 | 0.00246 |
| | $HO^+$ | $X^3\Sigma^-$ | 1.0289 | 0.00134 | 0.00133 | 0.00133 | 0.00132 | 0.00133 | 0.00132 | 0.00131 | 0.00132 |
| | $O_2$ | $X^3\Sigma_g^-$ | 1.20752 | 0.00340 | 0.00335 | 0.00336 | 0.00337 | 0.00333 | 0.00335 | 0.00333 | 0.00334 |
| | $O_2^+$ | $X^2\Pi_g$ | 1.1164 | -0.00158 | 0.00227 | 0.00226 | 0.00235 | 0.00227 | 0.00230 | 0.00228 | 0.00229 |
| | $O_2^-$ | $X^2\Pi_{g,i}$ | 1.35 | 0.00396 | 0.00373 | 0.00374 | 0.00361 | 0.00365 | 0.00370 | 0.00371 | 0.00370 |
| | OF | $X^2\Pi$ | 1.35411 | 0.00324 | 0.00492 | 0.00508 | 0.00516 | 0.00459 | 0.00472 | 0.00466 | 0.00463 |
| | $HF^+$ | $X^2\Pi_i$ | 1.00105 | 0.00302 | 0.00302 | 0.00302 | 0.00302 | 0.00299 | 0.00300 | 0.00300 | 0.00301 |
| | $F_2^+$ | $X^2\Pi_{g,i}$ | 1.3119 | -0.00197 | -0.00024 | -0.00058 | -0.00024 | -0.00014 | -0.00001 | 0.00009 | 0.00011 |
| | $F_2^-$ | $X^2\Sigma_u^+$ | 1.88 | 0.03882 | 0.04568 | 0.04590 | 0.04528 | 0.04553 | 0.04555 | 0.04553 | 0.04544 |
| | RMSD | | | 0.01562 | 0.01410 | 0.01413 | 0.01419 | 0.01406 | 0.01406 | 0.01404 | 0.01408 |
| | MSD | | | 0.00635 | 0.00621 | 0.00651 | 0.00691 | 0.00656 | 0.00654 | 0.00636 | 0.00662 |
| | MIN | | | -0.00741 | -0.00463 | -0.00209 | -0.00173 | -0.00199 | -0.00203 | -0.00211 | -0.00207 |
| | MAX | | | 0.04824 | 0.04909 | 0.04915 | 0.04917 | 0.04909 | 0.04908 | 0.04912 | 0.04914 |
| Row 2–Row 3 | Dimer | State | Expt. | Δ(CCSD(T): UHF) | Δ(CCSD(T): κ-OOMP2) | Δ(CCSD(T): OOMP2) | Δ(CCSD(T): BLYP) | Δ(CCSD(T): B97M-rV) | Δ(CCSD(T): B97) | Δ(CCSD(T): ωB97X-V) | Δ(CCSD(T): ωB97M-V) |
| | MgH | $X^2\Sigma^+$ | 1.7297 | 0.00203 | 0.00201 | 0.00201 | 0.00242 | 0.00209 | 0.00229 | 0.00220 | 0.00211 |
| | MgF | $X^2\Sigma^+$ | 1.75 | 0.00585 | 0.00605 | 0.00618 | 0.00658 | 0.00628 | 0.00629 | 0.00617 | 0.00616 |

| | | | | | | | | | | |
|---|---|---|---|---|---|---|---|---|---|---|
| | $AlH^+$ | $X^2\Sigma^+$ | 1.6018 | 0.00589 | 0.00583 | 0.00582 | 0.00586 | 0.00581 | 0.00582 | 0.00583 | 0.00582 |
| | SiH | $X^2\Pi_r$ | 1.5201 | 0.00085 | 0.00030 | 0.00031 | 0.00035 | 0.00037 | 0.00033 | 0.00032 | 0.00035 |
| | SiF | $X^2\Pi_r$ | 1.6011 | 0.00604 | 0.00638 | 0.00657 | 0.00700 | 0.00662 | 0.00662 | 0.00647 | 0.00650 |
| | PH | $X^3\Sigma^-$ | 1.42234 | -0.00007 | -0.00006 | -0.00006 | -0.00004 | -0.00004 | -0.00005 | -0.00006 | -0.00005 |
| | $PH^+$ | $X^2\Pi_r$ | 1.4352 | -0.01149 | -0.01153 | -0.01153 | -0.01149 | -0.01149 | -0.01151 | -0.01151 | -0.01150 |
| | $PH^-$ | $X^2\Pi_i$ | 1.407 | 0.02776 | 0.02776 | 0.02777 | 0.02781 | 0.02777 | 0.02780 | 0.02778 | 0.02780 |
| | CP | $X^2\Sigma^+$ | 1.5622 | -0.00410 | 0.00333 | 0.00491 | 0.00447 | 0.00362 | 0.00385 | 0.00334 | 0.00368 |
| | PO | $X^2\Pi_r$ | 1.4759 | 0.00602 | 0.00626 | 0.00649 | 0.00639 | 0.00619 | 0.00618 | 0.00608 | 0.00609 |
| | $PO^-$ | $X^3\Sigma^-$ | 1.54 | 0.00107 | 0.00158 | 0.00198 | 0.00159 | 0.00139 | 0.00134 | 0.00126 | 0.00133 |
| | PF | $X^3\Sigma^-$ | 1.5897 | 0.00616 | 0.00652 | 0.00671 | 0.00711 | 0.00667 | 0.00670 | 0.00658 | 0.00660 |
| | $PF^+$ | $X^2\Pi_r$ | 1.5003 | 0.00642 | 0.00685 | 0.00712 | 0.00754 | 0.00707 | 0.00707 | 0.00688 | 0.00691 |
| | HS | $X^2\Pi_i$ | 1.3409 | -0.00046 | -0.00044 | -0.00044 | -0.00043 | -0.00043 | -0.00042 | -0.00043 | -0.00043 |
| | BS | $X^2\Sigma^+$ | 1.6092 | 0.00431 | 0.00519 | 0.00540 | 0.00559 | 0.00536 | 0.00542 | 0.00531 | 0.00532 |
| | $CS^+$ | $X^2\Sigma^+$ | 1.4954 | -0.00616 | 0.00048 | 0.00154 | 0.00137 | 0.00044 | 0.00078 | 0.00052 | 0.00067 |
| | NS | $X^2\Pi_r$ | 1.49402 | -0.00140 | 0.00501 | 0.00512 | 0.00515 | 0.00500 | 0.00500 | 0.00492 | 0.00498 |
| | SO | $X^3\Sigma^-$ | 1.48109 | 0.00498 | 0.00559 | 0.00578 | 0.00539 | 0.00519 | 0.00523 | 0.00520 | 0.00522 |
| | $SO^+$ | $X^2\Pi_r$ | 1.424 | -0.00047 | 0.00617 | 0.00629 | 0.00605 | 0.00588 | 0.00591 | 0.00586 | 0.00586 |
| | $HCl^+$ | $X^2\Pi_i$ | 1.31468 | -0.00149 | -0.00147 | -0.00147 | -0.00147 | -0.00146 | -0.00147 | -0.00147 | -0.00147 |
| | BeCl | $X^2\Sigma^+$ | 1.7971 | 0.00604 | 0.00606 | 0.00609 | 0.00621 | 0.00618 | 0.00613 | 0.00607 | 0.00610 |
| | CCl | $X^2\Pi$ | 1.645 | 0.00576 | 0.00609 | 0.00672 | 0.00708 | 0.00655 | 0.00656 | 0.00614 | 0.00624 |
| | NCl | $X^3\Sigma^-$ | 1.6144 | 0.00466 | 0.00475 | 0.00537 | 0.00568 | 0.00510 | 0.00516 | 0.00487 | 0.00487 |
| | OCl | $X^2\Pi_i$ | 1.56963 | 0.00581 | 0.00644 | 0.00647 | 0.00646 | 0.00654 | 0.00652 | 0.00649 | 0.00650 |
| | RMSD | | | 0.00752 | 0.00770 | 0.00784 | 0.00790 | 0.00775 | 0.00776 | 0.00769 | 0.00771 |
| | MSD | | | 0.00308 | 0.00438 | 0.00463 | 0.00469 | 0.00445 | 0.00448 | 0.00437 | 0.00440 |
| | MIN | | | -0.01149 | -0.01153 | -0.01153 | -0.01149 | -0.01149 | -0.01151 | -0.01151 | -0.01150 |
| | MAX | | | 0.02776 | 0.02776 | 0.02777 | 0.02781 | 0.02777 | 0.02780 | 0.02778 | 0.02780 |

| Row 3–Row 3 | Dimer | State | Expt. | Δ(CCSD(T): UHF) | Δ(CCSD(T): κ-OOMP2) | Δ(CCSD(T): OOMP2) | Δ(CCSD(T): BLYP) | Δ(CCSD(T): B97M-rV) | Δ(CCSD(T): B97) | Δ(CCSD(T): ωB97X-V) | Δ(CCSD(T): ωB97M-V) |
|---|---|---|---|---|---|---|---|---|---|---|---|
| | MgCl | $X^2\Sigma^+$ | 2.1991 | 0.00793 | 0.00792 | 0.00793 | 0.00806 | 0.00798 | 0.00800 | 0.00797 | 0.00790 |
| | AlS | $X^2\Sigma^+$ | 2.029 | 0.01279 | 0.01346 | 0.01411 | 0.01355 | 0.01368 | 0.01342 | 0.01305 | 0.01291 |
| | $Si_2$ | $X^3\Sigma_g^-$ | 2.246 | 0.00857 | 0.00846 | -0.07907 | 0.00844 | 0.00841 | 0.00840 | 0.00842 | 0.00839 |
| | SiCl | $X^2\Pi_r$ | 2.058 | 0.01415 | 0.01415 | 0.01432 | 0.01467 | 0.01444 | 0.01437 | 0.01417 | 0.01422 |
| | ${P_2}^+$ | $X^2\Pi_u$ | 1.9859 | -0.01283 | -0.00204 | -0.08190 | -0.00214 | -0.00220 | -0.00216 | -0.00207 | -0.00206 |
| | PS | $X^2\Pi_r$ | 1.9009 | -0.00514 | 0.00596 | 0.00606 | 0.00606 | 0.00601 | 0.00597 | 0.00597 | 0.00597 |
| | $S_2$ | $X^3\Sigma_g^-$ | 1.8892 | 0.01018 | 0.01007 | 0.01019 | 0.01007 | 0.01004 | 0.01004 | 0.01004 | 0.01004 |
| | ${S_2}^+$ | $X^2\Pi_{g,r}$ | 1.825 | -0.00387 | 0.00687 | 0.00694 | 0.00685 | 0.00679 | 0.00681 | 0.00684 | 0.00684 |
| | RMSD | | | 0.01006 | 0.00938 | 0.04125 | 0.00952 | 0.00947 | 0.00941 | 0.00931 | 0.00928 |
| | MSD | | | 0.00397 | 0.00811 | -0.01268 | 0.00820 | 0.00814 | 0.00811 | 0.00805 | 0.00803 |
| | MIN | | | -0.01283 | -0.00204 | -0.08190 | -0.00214 | -0.00220 | -0.00216 | -0.00207 | -0.00206 |
| | MAX | | | 0.01415 | 0.01415 | 0.01432 | 0.01467 | 0.01444 | 0.01437 | 0.01417 | 0.01422 |

| Open-shell | Dimer | State | Expt. | Δ(CCSD(T): UHF) | Δ(CCSD(T): $\kappa$-OOMP2) | Δ(CCSD(T): OOMP2) | Δ(CCSD(T): BLYP) | Δ(CCSD(T): B97M-rV) | Δ(CCSD(T): B97) | Δ(CCSD(T): $\omega$B97X-V) | Δ(CCSD(T): $\omega$B97M-V) |
|---|---|---|---|---|---|---|---|---|---|---|---|
| | RMSD | | | 0.01197 | 0.01110 | 0.01884 | 0.01122 | 0.01110 | 0.01110 | 0.01106 | 0.01108 |
| | MSD | | | 0.00506 | 0.00611 | 0.00395 | 0.00655 | 0.00629 | 0.00629 | 0.00616 | 0.00629 |
| | MIN | | | -0.01283 | -0.01153 | -0.08190 | -0.01149 | -0.01149 | -0.01151 | -0.01151 | -0.01150 |
| | MAX | | | 0.04824 | 0.04909 | 0.04915 | 0.04917 | 0.04909 | 0.04908 | 0.04912 | 0.04914 |

Table S4: Root mean square deviations, mean signed deviations, most negative deviation, and most positive deviations in the equilibrium bond lengths for all species are are presented for the CCSD methods utilizing different molecular orbital references.

| | Δ(CCSD: UHF) | Δ(CCSD: κ-OOMP2) | Δ(CCSD: OOMP2) | Δ(CCSD: BLYP) | Δ(CCSD: B97M-rV) | Δ(CCSD: B97) | Δ(CCSD: ωB97X-V) | Δ(CCSD: ωB97M-V) |
|---|---|---|---|---|---|---|---|---|
| RMSD | 0.02276 | 0.01352 | 0.020060 | 0.01465 | 0.01442 | 0.01445 | 0.01435 | 0.01437 |
| MSD | -0.00021 | -0.00259 | -0.00454 | -0.00245 | -0.00202 | -0.00205 | -0.00177 | -0.00182 |
| MIN | -0.03572 | -0.02706 | -0.10195 | -0.02699 | -0.02629 | -0.02621 | -0.02596 | -0.02589 |
| MAX | 0.17058 | 0.08265 | 0.08996 | 0.08987 | 0.08983 | 0.09008 | 0.09041 | 0.08989 |

Table S5: Experimental equilibrium bond lengths (in Å) and errors in the computed bond lengths (in Å) for the closed-shell species are presented for the CCSD methods utilizing different molecular orbitals. Root mean square deviations, mean signed deviations, most negative deviations, and most positive deviations (all in Å) for the set of species and subsets are presented. Experimental values were compiled by Huber and Herzberg **?** .

| Row 2–Row 2 | Dimer | State | Expt. | Δ(CCSD: UHF) | Δ(CCSD: κ-OOMP2) | Δ(CCSD: OOMP2) | Δ(CCSD: BLYP) | Δ(CCSD: B97M-rV) | Δ(CCSD: B97) | Δ(CCSD: ωB97X-V) | Δ(CCSD: ωB97M-V) |
|---|---|---|---|---|---|---|---|---|---|---|---|
| | LiH | $X^1\Sigma^+$ | 1.5957 | 0.00203 | 0.00204 | 0.00203 | 0.00203 | 0.00201 | 0.00203 | 0.00204 | 0.00204 |
| | $Li_2$ | $X^1\Sigma_g^+$ | 2.6729 | 0.00946 | 0.00748 | 0.00746 | 0.00735 | 0.00711 | 0.00737 | 0.00747 | 0.00743 |
| | LiF | $X^1\Sigma^+$ | 1.56386 | 0.00041 | -0.00048 | -0.00073 | -0.00097 | -0.00059 | -0.00060 | -0.00054 | -0.00061 |
| | $BeH^+$ | $X^1\Sigma^+$ | 1.3122 | 0.00001 | 0.00001 | 0.00000 | 0.00000 | 0.00002 | 0.00000 | 0.00000 | 0.00000 |
| | BeO | $X^1\Sigma^+$ | 1.3309 | -0.00998 | -0.01298 | -0.01468 | -0.01405 | -0.01310 | -0.01331 | -0.01256 | -0.01281 |
| | BH | $X^1\Sigma^+$ | 1.2324 | -0.00180 | -0.00168 | -0.00215 | -0.00211 | -0.00210 | -0.00226 | -0.00221 | -0.00220 |
| | BF | $X^1\Sigma^+$ | 1.26259 | 0.00188 | 0.00081 | 0.00063 | 0.00028 | 0.00073 | 0.00063 | 0.00074 | 0.00070 |
| | $C_2$ | $X^1\Sigma_g^+$ | 1.24253 | -0.01475 | -0.01391 | -0.00579 | 0.03649 | 0.03668 | 0.03615 | 0.03636 | 0.03743 |
| | CO | $X^1\Sigma^+$ | 1.12832 | -0.00318 | -0.00443 | -0.00463 | -0.00470 | -0.00431 | -0.00437 | -0.00423 | -0.00424 |
| | $N_2$ | $X^1\Sigma_g^+$ | 1.09769 | -0.00473 | -0.00565 | -0.00580 | -0.00584 | -0.00551 | -0.00559 | -0.00544 | -0.00545 |
| | $NO^+$ | $X^1\Sigma^+$ | 1.06322 | -0.00638 | -0.00775 | -0.00792 | -0.00790 | -0.00750 | -0.00757 | -0.00742 | -0.00742 |
| | $OH^-$ | $X^1\Sigma^+$ | 0.97 | -0.00732 | -0.00821 | -0.00854 | -0.00826 | -0.00803 | -0.00802 | -0.00793 | -0.00796 |
| | HF | $X^1\Sigma^+$ | 0.91681 | 0.00062 | 0.00019 | 0.00014 | 0.00005 | 0.00027 | 0.00022 | 0.00022 | 0.00020 |
| | $F_2$ | $X^1\Sigma_g^+$ | 1.41193 | -0.03572 | -0.02017 | -0.02067 | -0.02037 | -0.01982 | -0.01987 | -0.01972 | -0.01969 |
| | RMSD | | | 0.01140 | 0.00850 | 0.00816 | 0.01252 | 0.01236 | 0.01229 | 0.01225 | 0.01249 |
| | MSD | | | -0.00496 | -0.00462 | -0.00433 | -0.00129 | -0.00101 | -0.00109 | -0.00094 | -0.00090 |
| | MIN | | | -0.03572 | -0.02017 | -0.02067 | -0.02037 | -0.01982 | -0.01987 | -0.01972 | -0.01969 |
| | MAX | | | 0.00946 | 0.00748 | 0.00746 | 0.03649 | 0.03668 | 0.03615 | 0.03636 | 0.03743 |
| Row 2–Row 3 | Dimer | State | Expt. | Δ(CCSD: UHF) | Δ(CCSD: κ-OOMP2) | Δ(CCSD: OOMP2) | Δ(CCSD: BLYP) | Δ(CCSD: B97M-rV) | Δ(CCSD: B97) | Δ(CCSD: ωB97X-V) | Δ(CCSD: ωB97M-V) |
| | NaH | $X^1\Sigma^+$ | 1.8874 | 0.00651 | 0.00674 | 0.00671 | 0.00700 | 0.00677 | 0.00685 | 0.00698 | 0.00694 |
| | NaLi | $X^1\Sigma^+$ | 2.81 | 0.08327 | 0.08265 | 0.08996 | 0.08987 | 0.08983 | 0.09008 | 0.09041 | 0.08989 |
| | NaF | $X^1\Sigma^+$ | 1.92595 | 0.00475 | 0.00380 | 0.00346 | 0.00338 | 0.00364 | 0.00369 | 0.00382 | 0.00373 |
| | $MgH^+$ | $X^1\Sigma^+$ | 1.6519 | 0.00236 | 0.00239 | 0.00233 | 0.00259 | 0.00236 | 0.00250 | 0.00254 | 0.00243 |
| | AlH | $X^1\Sigma^+$ | 1.6478 | -0.00022 | -0.00130 | -0.00136 | -0.00150 | -0.00131 | -0.00145 | -0.00132 | -0.00133 |
| | AlF | $X^1\Sigma^+$ | 1.65437 | 0.00093 | -0.00018 | -0.00044 | -0.00083 | -0.00029 | -0.00041 | -0.00027 | -0.00032 |
| | $SiH^+$ | $X^1\Sigma^+$ | 1.5041 | -0.00247 | -0.00290 | -0.00293 | -0.00299 | -0.00293 | -0.00295 | -0.00289 | -0.00289 |
| | SiO | $X^1\Sigma^+$ | 1.50974 | -0.00615 | -0.00802 | -0.00892 | -0.00862 | -0.00816 | -0.00816 | -0.00775 | -0.00778 |
| | PN | $X^1\Sigma^+$ | 1.49087 | -0.01339 | -0.01050 | -0.01150 | -0.01088 | -0.01047 | -0.01042 | -0.01002 | -0.01001 |
| | BeS | $X^1\Sigma^+$ | 1.74153 | 0.17058 | -0.00488 | -0.00585 | -0.00611 | -0.00551 | -0.00559 | -0.00488 | -0.00507 |
| | CS | $X^1\Sigma^+$ | 1.53494 | -0.00762 | -0.00962 | -0.01049 | -0.01026 | -0.00969 | -0.00976 | -0.00921 | -0.00932 |
| | $NS^+$ | $X^1\Sigma^+$ | 1.44 | -0.01821 | -0.01577 | -0.01669 | -0.01611 | -0.01558 | -0.01560 | -0.01519 | -0.01523 |

| | | | | | | | | | | |
|---|---|---|---|---|---|---|---|---|---|---|
| | HCl | $X^1\Sigma^+$ | 1.27455 | -0.00306 | -0.00319 | -0.00324 | -0.00330 | -0.00320 | -0.00323 | -0.00316 | -0.00322 |
| | LiCl | $X^1\Sigma^+$ | 2.02067 | 0.00558 | 0.00549 | 0.00538 | 0.00517 | 0.00536 | 0.00535 | 0.00542 | 0.00534 |
| | BCl | $X^1\Sigma^+$ | 1.7159 | 0.00065 | 0.00024 | -0.00024 | -0.00090 | -0.00046 | -0.00041 | 0.00005 | -0.00007 |
| | ClF | $X^1\Sigma^+$ | 1.62831 | -0.00640 | -0.00772 | -0.00807 | -0.00799 | -0.00748 | -0.00756 | -0.00739 | -0.00742 |
| | RMSD | | | 0.04796 | 0.02172 | 0.02359 | 0.02352 | 0.02343 | 0.02350 | 0.02352 | 0.02340 |
| | MSD | | | 0.01357 | 0.00233 | 0.00238 | 0.00241 | 0.00268 | 0.00268 | 0.00295 | 0.00285 |
| | MIN | | | -0.01821 | -0.01577 | -0.01669 | -0.01611 | -0.01558 | -0.01560 | -0.01519 | -0.01523 |
| | MAX | | | 0.17058 | 0.08265 | 0.08996 | 0.08987 | 0.08983 | 0.09008 | 0.09041 | 0.08989 |
| Row 3–Row 3 | Dimer | State | Expt. | Δ(CCSD: UHF) | Δ(CCSD: $\kappa$-OOMP2) | Δ(CCSD: OOMP2) | Δ(CCSD: BLYP) | Δ(CCSD: B97M-rV) | Δ(CCSD: B97) | Δ(CCSD: $\omega$B97X-V) | Δ(CCSD: $\omega$B97M-V) |
| | NaCl | $X^1\Sigma^+$ | 2.36079 | 0.01274 | 0.01276 | 0.01265 | 0.01259 | 0.01265 | 0.01269 | 0.01281 | 0.01272 |
| | AlCl | $X^1\Sigma^+$ | 2.13011 | 0.01222 | 0.01200 | 0.01174 | 0.01126 | 0.01164 | 0.01158 | 0.01184 | 0.01178 |
| | SiS | $X^1\Sigma^+$ | 1.92932 | -0.00253 | -0.00378 | -0.00481 | -0.00500 | -0.00447 | -0.00448 | -0.00376 | -0.00390 |
| | $P_2$ | $X^1\Sigma_g^+$ | 1.8934 | -0.01803 | -0.00962 | -0.01062 | -0.01054 | -0.01009 | -0.01012 | -0.00945 | -0.00949 |
| | $Cl_2$ | $X^1\Sigma_g^+$ | 1.9879 | 0.00599 | 0.00566 | 0.00544 | 0.00526 | 0.00556 | 0.00556 | 0.00567 | 0.00563 |
| | RMSD | | | 0.01165 | 0.00944 | 0.00963 | 0.00948 | 0.00947 | 0.00947 | 0.00938 | 0.00935 |
| | MSD | | | 0.00208 | 0.00340 | 0.00288 | 0.00271 | 0.00306 | 0.00305 | 0.00342 | 0.00335 |
| | MIN | | | -0.01803 | -0.00962 | -0.01062 | -0.01054 | -0.01009 | -0.01012 | -0.00945 | -0.00949 |
| | MAX | | | 0.01274 | 0.01276 | 0.01265 | 0.01259 | 0.01265 | 0.01269 | 0.01281 | 0.01272 |
| Closed-shell | | | | Δ(CCSD: UHF) | Δ(CCSD: $\kappa$-OOMP2) | Δ(CCSD: OOMP2) | Δ(CCSD: BLYP) | Δ(CCSD: B97M-rV) | Δ(CCSD: B97) | Δ(CCSD: $\omega$B97X-V) | Δ(CCSD: $\omega$B97M-V) |
| | RMSD | | | 0.03351 | 0.01604 | 0.01716 | 0.01812 | 0.01802 | 0.01805 | 0.01804 | 0.01803 |
| | MSD | | | 0.00452 | -0.00030 | -0.00023 | 0.00097 | 0.00126 | 0.00123 | 0.00146 | 0.00142 |
| | MIN | | | -0.03572 | -0.02017 | -0.02067 | -0.02037 | -0.01982 | -0.01987 | -0.01972 | -0.01969 |
| | MAX | | | 0.17058 | 0.08265 | 0.08996 | 0.08987 | 0.08983 | 0.09008 | 0.09041 | 0.08989 |

Table S6: Experimental equilibrium bond lengths (in Å) and errors in the computed bond lengths (in Å) for the open-shell species are presented for the CCSD methods utilizing different molecular orbitals. Root mean square deviations, mean signed deviations, most negative deviations, and most positive deviations (all in Å) for the set of species and subsets are presented. Experimental values were compiled by Huber and Herzberg **?** .

| Row 2–Row 2 | Dimer | State | Expt. | Δ(CCSD: UHF) | Δ(CCSD: κ-OOMP2) | Δ(CCSD: OOMP2) | Δ(CCSD: BLYP) | Δ(CCSD: B97M-rV) | Δ(CCSD: B97) | Δ(CCSD: ωB97X-V) | Δ(CCSD: ωB97M-V) |
|---|---|---|---|---|---|---|---|---|---|---|---|
| | LiO | $X^2\Pi_i$ | 1.695 | -0.00729 | -0.00808 | -0.00846 | -0.00889 | -0.00844 | -0.00844 | -0.00828 | -0.00842 |
| | BeH | $X^2\Sigma^+$ | 1.3426 | -0.00045 | -0.00051 | -0.00051 | -0.00054 | -0.00045 | -0.00054 | -0.00053 | -0.00054 |
| | BeF | $X^2\Sigma^+$ | 1.361 | 0.00033 | -0.00042 | -0.00056 | -0.00085 | -0.00049 | -0.00054 | -0.00048 | -0.00054 |
| | $B_2$ | $X^3\Sigma_g^-$ | 1.59 | -0.02379 | -0.02361 | -0.00059 | -0.02699 | -0.02375 | -0.02397 | -0.02270 | -0.02356 |
| | BN | $X^3\Pi$ | 1.281 | 0.03714 | 0.03588 | 0.03526 | 0.03517 | 0.03575 | 0.03578 | 0.03600 | 0.03581 |
| | BO | $X^2\Sigma^+$ | 1.2045 | -0.00266 | -0.00412 | -0.00455 | -0.00470 | -0.00420 | -0.00436 | -0.00407 | -0.00411 |
| | CH | $X^2\Pi_r$ | 1.1199 | -0.00108 | -0.00185 | -0.00187 | -0.00200 | -0.00186 | -0.00193 | -0.00187 | -0.00192 |
| | $C_2^-$ | $X^2\Sigma_g^+$ | 1.26821 | 0.03456 | -0.00645 | -0.00720 | -0.00663 | -0.00613 | -0.00624 | -0.00608 | -0.00579 |
| | CN | $X^2\Sigma^+$ | 1.17182 | -0.00895 | -0.00851 | -0.00865 | -0.00830 | -0.00805 | -0.00816 | -0.00805 | -0.00825 |
| | $CO^+$ | $X^2\Sigma^+$ | 1.11522 | -0.00599 | -0.00804 | -0.00855 | -0.00849 | -0.00771 | -0.00793 | -0.00774 | -0.00773 |
| | CF | $X^2\Pi_r$ | 1.2718 | -0.00126 | -0.00325 | -0.00361 | -0.00402 | -0.00339 | -0.00341 | -0.00321 | -0.00325 |
| | NH | $X^3\Sigma^-$ | 1.03621 | -0.00064 | -0.00087 | -0.00090 | -0.00102 | -0.00089 | -0.00090 | -0.00088 | -0.00092 |
| | $N_2^+$ | $X^2\Sigma_g^+$ | 1.11642 | -0.00980 | -0.00828 | -0.00899 | -0.00819 | -0.00764 | -0.00773 | -0.00745 | -0.00752 |
| | NO | $X^2\Pi_r$ | 1.15077 | -0.00682 | -0.00878 | -0.00907 | -0.00899 | -0.00852 | -0.00860 | -0.00842 | -0.00844 |
| | NF | $X^3\Sigma^-$ | 1.31698 | -0.00409 | -0.00726 | -0.00797 | -0.00844 | -0.00722 | -0.00735 | -0.00700 | -0.00696 |
| | OH | $X^2\Pi_i$ | 0.96966 | -0.00029 | -0.00061 | -0.00066 | -0.00075 | -0.00061 | -0.00061 | -0.00060 | -0.00063 |
| | $HO^+$ | $X^3\Sigma^-$ | 1.0289 | -0.00101 | -0.00117 | -0.00118 | -0.00133 | -0.00126 | -0.00122 | -0.00124 | -0.00126 |
| | $O_2$ | $X^3\Sigma_g^-$ | 1.20752 | -0.00845 | -0.01060 | -0.01101 | -0.01075 | -0.01022 | -0.01023 | -0.01006 | -0.01009 |
| | $O_2^+$ | $X^2\Pi_g$ | 1.1164 | -0.01172 | -0.01209 | -0.01243 | -0.01216 | -0.01167 | -0.01172 | -0.01152 | -0.01154 |
| | $O_2^-$ | $X^2\Pi_{g,i}$ | 1.35 | -0.01316 | -0.01649 | -0.01747 | -0.01637 | -0.01565 | -0.01566 | -0.01552 | -0.01552 |
| | OF | $X^2\Pi$ | 1.35411 | -0.00842 | -0.01446 | -0.01657 | -0.01550 | -0.01338 | -0.01356 | -0.01296 | -0.01283 |
| | $HF^+$ | $X^2\Pi_i$ | 1.00105 | 0.00023 | -0.00003 | -0.00005 | -0.00025 | -0.00005 | -0.00011 | -0.00013 | -0.00013 |
| | $F_2^+$ | $X^2\Pi_{g,i}$ | 1.3119 | -0.02617 | -0.02706 | -0.02809 | -0.02695 | -0.02629 | -0.02621 | -0.02596 | -0.02589 |
| | $F_2^-$ | $X^2\Sigma_u^+$ | 1.88 | 0.00653 | 0.03413 | 0.03232 | 0.03358 | 0.03458 | 0.03461 | 0.03464 | 0.03463 |
| | RMSD | | | 0.01393 | 0.01437 | 0.01365 | 0.01461 | 0.01421 | 0.01425 | 0.01409 | 0.01413 |
| | MSD | | | -0.00264 | -0.00427 | -0.00381 | -0.00472 | -0.00406 | -0.00413 | -0.00392 | -0.00398 |
| | MIN | | | -0.02617 | -0.02706 | -0.02809 | -0.02699 | -0.02629 | -0.02621 | -0.02596 | -0.02589 |
| | MAX | | | 0.03714 | 0.03588 | 0.03526 | 0.03517 | 0.03575 | 0.03578 | 0.03600 | 0.03581 |
| Row 2–Row 3 | Dimer | State | Expt. | Δ(CCSD: UHF) | Δ(CCSD: κ-OOMP2) | Δ(CCSD: OOMP2) | Δ(CCSD: BLYP) | Δ(CCSD: B97M-rV) | Δ(CCSD: B97) | Δ(CCSD: ωB97X-V) | Δ(CCSD: ωB97M-V) |
| | MgH | $X^2\Sigma^+$ | 1.7297 | 0.00074 | 0.00060 | 0.00054 | 0.00089 | 0.00055 | 0.00082 | 0.00076 | 0.00064 |
| | MgF | $X^2\Sigma^+$ | 1.75 | 0.00142 | 0.00045 | 0.00019 | -0.00003 | 0.00024 | 0.00028 | 0.00041 | 0.00031 |

| | | | | | | | | | | |
|---|---|---|---|---|---|---|---|---|---|---|
| | AlH$^+$ | $X^2\Sigma^+$ | 1.6018 | 0.00274 | 0.00223 | 0.00210 | 0.00194 | 0.00200 | 0.00198 | 0.00206 | 0.00206 |
| | SiH | $X^2\Pi_r$ | 1.5201 | -0.00073 | -0.00200 | -0.00206 | -0.00217 | -0.00209 | -0.00211 | -0.00200 | -0.00203 |
| | SiF | $X^2\Pi_r$ | 1.6011 | 0.00007 | -0.00129 | -0.00160 | -0.00204 | -0.00150 | -0.00155 | -0.00138 | -0.00141 |
| | PH | $X^3\Sigma^-$ | 1.42234 | -0.00307 | -0.00315 | -0.00321 | -0.00329 | -0.00321 | -0.00324 | -0.00314 | -0.00319 |
| | PH$^+$ | $X^2\Pi_r$ | 1.4352 | -0.01396 | -0.01406 | -0.01409 | -0.01414 | -0.01409 | -0.01412 | -0.01405 | -0.01409 |
| | PH$^-$ | $X^2\Pi_i$ | 1.407 | 0.02464 | 0.02448 | 0.02432 | 0.02420 | 0.02434 | 0.02431 | 0.02452 | 0.02441 |
| | CP | $X^2\Sigma^+$ | 1.5622 | -0.01089 | -0.01033 | -0.01285 | -0.01147 | -0.01050 | -0.01059 | -0.00990 | -0.01018 |
| | PO | $X^2\Pi_r$ | 1.4759 | -0.00649 | -0.00840 | -0.00917 | -0.00890 | -0.00848 | -0.00842 | -0.00810 | -0.00810 |
| | PO$^-$ | $X^3\Sigma^-$ | 1.54 | -0.00968 | -0.01166 | -0.01253 | -0.01222 | -0.01182 | -0.01167 | -0.01136 | -0.01144 |
| | PF | $X^3\Sigma^-$ | 1.5897 | -0.00123 | -0.00281 | -0.00319 | -0.00372 | -0.00307 | -0.00311 | -0.00291 | -0.00291 |
| | PF$^+$ | $X^2\Pi_r$ | 1.5003 | -0.00140 | -0.00341 | -0.00386 | -0.00423 | -0.00363 | -0.00365 | -0.00340 | -0.00341 |
| | HS | $X^2\Pi_i$ | 1.3409 | -0.00320 | -0.00333 | -0.00339 | -0.00346 | -0.00339 | -0.00341 | -0.00330 | -0.00337 |
| | BS | $X^2\Sigma^+$ | 1.6092 | -0.00411 | -0.00513 | -0.00578 | -0.00604 | -0.00547 | -0.00558 | -0.00507 | -0.00525 |
| | CS$^+$ | $X^2\Sigma^+$ | 1.4954 | -0.01279 | -0.01351 | -0.01497 | -0.01452 | -0.01346 | -0.01370 | -0.01313 | -0.01335 |
| | NS | $X^2\Pi_r$ | 1.49402 | -0.01009 | -0.01066 | -0.01193 | -0.01096 | -0.01033 | -0.01031 | -0.00982 | -0.00993 |
| | SO | $X^3\Sigma^-$ | 1.48109 | -0.00657 | -0.00856 | -0.00929 | -0.00873 | -0.00831 | -0.00821 | -0.00794 | -0.00799 |
| | SO$^+$ | $X^2\Pi_r$ | 1.424 | -0.01295 | -0.01122 | -0.01204 | -0.01149 | -0.01105 | -0.01099 | -0.01068 | -0.01068 |
| | HCl$^+$ | $X^2\Pi_i$ | 1.31468 | -0.00421 | -0.00426 | -0.00427 | -0.00430 | -0.00427 | -0.00425 | -0.00422 | -0.00428 |
| | BeCl | $X^2\Sigma^+$ | 1.7971 | 0.00404 | 0.00387 | 0.00373 | 0.00346 | 0.00365 | 0.00365 | 0.00380 | 0.00372 |
| | CCl | $X^2\Pi$ | 1.645 | 0.00099 | -0.00037 | -0.00139 | -0.00184 | -0.00116 | -0.00120 | -0.00044 | -0.00064 |
| | NCl | $X^3\Sigma^-$ | 1.6144 | 0.00039 | -0.00092 | -0.00249 | -0.00311 | -0.00186 | -0.00204 | -0.00120 | -0.00125 |
| | OCl | $X^2\Pi_i$ | 1.56963 | -0.00068 | -0.00504 | -0.00797 | -0.00621 | -0.00446 | -0.00481 | -0.00382 | -0.00394 |
| | RMSD | | | 0.00821 | 0.00852 | 0.00910 | 0.00883 | 0.00850 | 0.00851 | 0.00832 | 0.00836 |
| | MSD | | | -0.00279 | -0.00369 | -0.00438 | -0.00427 | -0.00381 | -0.00383 | -0.00351 | -0.00360 |
| | MIN | | | -0.01396 | -0.01406 | -0.01497 | -0.01452 | -0.01409 | -0.01412 | -0.01405 | -0.01409 |
| | MAX | | | 0.02464 | 0.02448 | 0.02432 | 0.02420 | 0.02434 | 0.02431 | 0.02452 | 0.02441 |

| Row 3–Row 3 | Dimer | State | Expt. | Δ(CCSD: UHF) | Δ(CCSD: $\kappa$-OOMP2) | Δ(CCSD: OOMP2) | Δ(CCSD: BLYP) | Δ(CCSD: B97M-rV) | Δ(CCSD: B97) | Δ(CCSD: $\omega$B97X-V) | Δ(CCSD: $\omega$B97M-V) |
|---|---|---|---|---|---|---|---|---|---|---|---|
| | MgCl | $X^2\Sigma^+$ | 2.1991 | 0.00554 | 0.00544 | 0.00530 | 0.00518 | 0.00524 | 0.00527 | 0.00542 | 0.00535 |
| | AlS | $X^2\Sigma^+$ | 2.029 | 0.00689 | 0.00444 | 0.00204 | 0.00352 | 0.00344 | 0.00404 | 0.00521 | 0.00518 |
| | $Si_2$ | $X^3\Sigma_g^-$ | 2.246 | -0.00635 | -0.00697 | -0.09502 | -0.00848 | -0.00771 | -0.00788 | -0.00715 | -0.00724 |
| | SiCl | $X^2\Pi_r$ | 2.058 | 0.01053 | 0.01015 | 0.00973 | 0.00914 | 0.00958 | 0.00959 | 0.00997 | 0.00988 |
| | $P_2^+$ | $X^2\Pi_u$ | 1.9859 | -0.02823 | -0.02187 | -0.10195 | -0.02310 | -0.02252 | -0.02263 | -0.02187 | -0.02196 |
| | PS | $X^2\Pi_r$ | 1.9009 | -0.01566 | -0.00996 | -0.01114 | -0.01116 | -0.01059 | -0.01063 | -0.00998 | -0.01009 |
| | $S_2$ | $X^3\Sigma_g^-$ | 1.8892 | -0.00251 | -0.00351 | -0.00423 | -0.00422 | -0.00385 | -0.00386 | -0.00339 | -0.00350 |
| | $S_2^+$ | $X^2\Pi_{g,r}$ | 1.825 | -0.01718 | -0.01185 | -0.01283 | -0.01262 | -0.01219 | -0.01222 | -0.01162 | -0.01171 |
| | RMSD | | | 0.01402 | 0.01079 | 0.04982 | 0.01135 | 0.01103 | 0.01111 | 0.01079 | 0.01083 |
| | MSD | | | -0.00587 | -0.00427 | -0.02601 | -0.00522 | -0.00483 | -0.00479 | -0.00418 | -0.00426 |
| | MIN | | | -0.02823 | -0.02187 | -0.10195 | -0.02310 | -0.02252 | -0.02263 | -0.02187 | -0.02196 |
| | MAX | | | 0.01053 | 0.01015 | 0.00973 | 0.00914 | 0.00958 | 0.00959 | 0.00997 | 0.00988 |

| Open-shell | | Δ(CCSD: UHF) | Δ(CCSD: $\kappa$-OOMP2) | Δ(CCSD: OOMP2) | Δ(CCSD: BLYP) | Δ(CCSD: B97M-rV) | Δ(CCSD: B97) | Δ(CCSD: $\omega$B97X-V) | Δ(CCSD: $\omega$B97M-V) |
|---|---|---|---|---|---|---|---|---|---|
| | RMSD | 0.01184 | 0.01167 | 0.02168 | 0.01197 | 0.01161 | 0.01165 | 0.01147 | 0.01150 |
| | MSD | -0.00317 | -0.00402 | -0.00723 | -0.00460 | -0.00406 | -0.00409 | -0.00378 | -0.00385 |
| | MIN | -0.02823 | -0.02706 | -0.10195 | -0.02699 | -0.02629 | -0.02621 | -0.02596 | -0.02589 |
| | MAX | 0.03714 | 0.03588 | 0.03526 | 0.03517 | 0.03575 | 0.03578 | 0.03600 | 0.03581 |

# 2 Species not included in the test set

Tab. S7 presents the species for which we were not able to obtain a continuous potential energy surface. For some cases this breakdown occurred at the SCF level with the reference curve changing character near equilibrium, leading to a discontinuous change in the CCSD energy. In other cases the $t$-amplitude optimization of CCSD was found to converge to different roots for different points along the surface.

Table S7: Species and experimental vibrational frequencies (in $cm^{-1}$) for which we were unable to compute a continuous PES with one or more of the methods surveyed. Experimental values were compiled by Huber and Herzberg **?** .

| Dimer | State | Expt. |
|---|---|---|
| $CH^-$ | $X^3\Sigma^-$ | 979.23 |
| $CN^+$ | $a^1\Sigma$ | 2033.05 |
| ${N_2}^-$ | $X^2\Pi_g$ | 1968 |
| MgO | $X^1\Sigma^+$ | 785.0 |
| AlN | $X^3\Pi_i$ | 746.93 |
| AlO | $X^2\Sigma^+$ | 979.23 |
| SiN | $X^2\Sigma^+$ | 1151.3 |
| $Na_2$ | $X^1\Sigma_g^+$ | 159.124 |
| ${Na_2}^+$ | $X^2\Sigma_g^+$ | 126 |
| $Mg_2$ | $X^1\Sigma_g^+$ | 51.12 |
| MgS | $X^1\Sigma^+$ | 528.74 |
| $Al_2$ | $X^3\Sigma_g^-$ | 350.01 |
| ${Cl_2}^+$ | $X^2\Pi_g$ | 645.61 |

# 3 Mean-field $\langle S^2 \rangle$ values

Table S8: Mean-field $\langle S^2 \rangle$ values for the reference methods at the CCSD(T) minimum energy points used in the fitting procedure.

| Closed-shell | Row 2–Row 2 | Dimer | State | CCSD(T): UHF | CCSD(T): $\kappa$-OOMP2 | CCSD(T): OOMP2 | CCSD(T): BLYP | CCSD(T): B97M-rV | CCSD(T): B97 | CCSD(T): $\omega$B97X-V | CCSD(T): $\omega$B97M-V |
|---|---|---|---|---|---|---|---|---|---|---|---|
| | | LiH | $X^1\Sigma^+$ | 0.00000 | 0.00000 | 0.00000 | 0.00000 | 0.00000 | 0.00000 | 0.00000 | 0.00000 |
| | | $Li_2$ | $X^1\Sigma_g^+$ | 0.31860 | 0.00000 | 0.00000 | 0.00000 | 0.01065 | 0.00000 | 0.00000 | 0.00000 |
| | | LiF | $X^1\Sigma^+$ | 0.00000 | 0.00000 | 0.00000 | 0.00000 | 0.00000 | 0.00000 | 0.00000 | 0.00000 |
| | | $BeH^+$ | $X^1\Sigma^+$ | 0.00000 | 0.00000 | 0.00000 | 0.00000 | 0.00000 | 0.00000 | 0.00000 | 0.00000 |
| | | BeO | $X^1\Sigma^+$ | 0.00000 | 0.00000 | 0.00000 | 0.00000 | 0.00000 | 0.00000 | 0.00000 | 0.00000 |
| | | BH | $X^1\Sigma^+$ | 0.47646 | 0.04871 | 0.00000 | 0.03506 | 0.00000 | 0.00000 | 0.00000 | 0.00000 |
| | | BF | $X^1\Sigma^+$ | 0.00000 | 0.00000 | 0.00000 | 0.00000 | 0.00000 | 0.00000 | 0.00000 | 0.00000 |
| | | $C_2$ | $X^1\Sigma_g^+$ | 1.65493 | 0.89140 | 0.00000 | 0.85447 | 0.94029 | 0.93904 | 1.01320 | 0.97020 |
| | | CO | $X^1\Sigma^+$ | 0.00000 | 0.00000 | 0.00000 | 0.00000 | 0.00000 | 0.00000 | 0.00000 | 0.00000 |
| | | $N_2$ | $X^1\Sigma_g^+$ | 0.00000 | 0.00000 | 0.00000 | 0.00000 | 0.00000 | 0.00000 | 0.00000 | 0.00000 |
| | | $NO^+$ | $X^1\Sigma^+$ | 0.00000 | 0.00000 | 0.00000 | 0.00000 | 0.00000 | 0.00000 | 0.00000 | 0.00000 |
| | | $OH^-$ | $X^1\Sigma^+$ | 0.00000 | 0.00000 | 0.00000 | 0.00000 | 0.00000 | 0.00000 | 0.00000 | 0.00000 |
| | | HF | $X^1\Sigma^+$ | 0.00000 | 0.00000 | 0.00000 | 0.00000 | 0.00000 | 0.00000 | 0.00000 | 0.00000 |
| | | $F_2$ | $X^1\Sigma_g^+$ | 0.31922 | 0.00000 | 0.00000 | 0.00000 | 0.00000 | 0.00000 | 0.00000 | 0.00000 |
| | Row 2–Row 3 | Dimer | State | CCSD(T): UHF | CCSD(T): $\kappa$-OOMP2 | CCSD(T): OOMP2 | CCSD(T): BLYP | CCSD(T): B97M-rV | CCSD(T): B97 | CCSD(T): $\omega$B97X-V | CCSD(T): $\omega$B97M-V |
| | | NaH | $X^1\Sigma^+$ | 0.00000 | 0.00000 | 0.00000 | 0.00000 | 0.00000 | 0.00000 | 0.00000 | 0.00000 |
| | | NaLi | $X^1\Sigma^+$ | 0.32431 | 0.03641 | 0.00000 | 0.00000 | 0.00000 | 0.00000 | 0.00000 | 0.00000 |
| | | NaF | $X^1\Sigma^+$ | 0.00000 | 0.00000 | 0.00000 | 0.00000 | 0.00000 | 0.00000 | 0.00000 | 0.00000 |
| | | $MgH^+$ | $X^1\Sigma^+$ | 0.00000 | 0.00000 | 0.00000 | 0.00000 | 0.00000 | 0.00000 | 0.00000 | 0.00000 |
| | | AlH | $X^1\Sigma^+$ | 0.17105 | 0.00000 | 0.00000 | 0.00000 | 0.00000 | 0.00000 | 0.00000 | 0.00000 |
| | | AlF | $X^1\Sigma^+$ | 0.00000 | 0.00000 | 0.00000 | 0.00000 | 0.00000 | 0.00000 | 0.00000 | 0.00000 |
| | | $SiH^+$ | $X^1\Sigma^+$ | 0.06997 | 0.00000 | 0.00000 | 0.00000 | 0.00000 | 0.00000 | 0.00000 | 0.00000 |
| | | SiO | $X^1\Sigma^+$ | 0.00000 | 0.00000 | 0.00000 | 0.00000 | 0.00000 | 0.00000 | 0.00000 | 0.00000 |
| | | PN | $X^1\Sigma^+$ | 0.70716 | 0.00000 | 0.00000 | 0.00000 | 0.00000 | 0.00000 | 0.00000 | 0.00000 |
| | | BeS | $X^1\Sigma^+$ | 1.01647 | 0.00000 | 0.00000 | 0.00000 | 0.00000 | 0.00000 | 0.00000 | 0.00000 |
| | | CS | $X^1\Sigma^+$ | 0.00000 | 0.00000 | 0.00000 | 0.00000 | 0.00000 | 0.00000 | 0.00000 | 0.00000 |
| | | $NS^+$ | $X^1\Sigma^+$ | 0.69154 | 0.00000 | 0.00000 | 0.00000 | 0.00000 | 0.00000 | 0.00000 | 0.00000 |
| | | HCl | $X^1\Sigma^+$ | 0.00000 | 0.00000 | 0.00000 | 0.00000 | 0.00000 | 0.00000 | 0.00000 | 0.00000 |
| | | LiCl | $X^1\Sigma^+$ | 0.00000 | 0.00000 | 0.00000 | 0.00000 | 0.00000 | 0.00000 | 0.00000 | 0.00000 |
| | | BCl | $X^1\Sigma^+$ | 0.17749 | 0.00000 | 0.00000 | 0.00000 | 0.00000 | 0.00000 | 0.00000 | 0.00000 |
| | | $CCl^+$ | $X^1\Sigma^+$ | 0.00000 | 0.00000 | 0.00000 | 0.00000 | 0.00000 | 0.00000 | 0.00000 | 0.00000 |
| | | ClF | $X^1\Sigma^+$ | 0.00000 | 0.00000 | 0.00000 | 0.00000 | 0.00000 | 0.00000 | 0.00000 | 0.00000 |
| | Row 3–Row 3 | Dimer | State | CCSD(T): UHF | CCSD(T): $\kappa$-OOMP2 | CCSD(T): OOMP2 | CCSD(T): BLYP | CCSD(T): B97M-rV | CCSD(T): B97 | CCSD(T): $\omega$B97X-V | CCSD(T): $\omega$B97M-V |
| | | NaCl | $X^1\Sigma^+$ | 0.00000 | 0.00000 | 0.00000 | 0.00000 | 0.00000 | 0.00000 | 0.00000 | 0.00000 |

| | | | | | | | | | | |
|---|---|---|---|---|---|---|---|---|---|---|
| | | AlCl | $X^1\Sigma^+$ | 0.00000 | 0.00000 | 0.00000 | 0.00000 | 0.00000 | 0.00000 | 0.00000 | 0.00000 |
| | | SiS | $X^1\Sigma^+$ | 0.00000 | 0.00000 | 0.00000 | 0.00000 | 0.00000 | 0.00000 | 0.00000 | 0.00000 |
| | | $P_2$ | $X^1\Sigma_g^+$ | 0.67604 | 0.00000 | 0.00000 | 0.00000 | 0.00000 | 0.00000 | 0.00000 | 0.00000 |
| | | $Cl_2$ | $X^1\Sigma_g^+$ | 0.00000 | 0.00000 | 0.00000 | 0.00000 | 0.00000 | 0.00000 | 0.00000 | 0.00000 |
| Open-shell | Row 2–Row2 | Dimer | State | CCSD(T): UHF | CCSD(T): $\kappa$-OOMP2 | CCSD(T): OOMP2 | CCSD(T): BLYP | CCSD(T): B97M-rV | CCSD(T): B97 | CCSD(T): $\omega$B97X-V | CCSD(T): $\omega$B97M-V |
| | | LiO | $X^2\Pi_i$ | 0.75970 | 0.75603 | 0.75612 | 0.75371 | 0.75619 | 0.75480 | 0.75372 | 0.75439 |
| | | BeH | $X^2\Sigma^+$ | 0.75204 | 0.75136 | 0.75144 | 0.75100 | 0.75042 | 0.75068 | 0.75107 | 0.75052 |
| | | BeF | $X^2\Sigma^+$ | 0.75083 | 0.75096 | 0.75103 | 0.75058 | 0.75212 | 0.75065 | 0.75065 | 0.75050 |
| | | $B_2$ | $X^3\Sigma_g^-$ | 2.90778 | 2.81206 | 2.00956 | 2.35395 | 2.47622 | 2.51071 | 2.90525 | 2.57710 |
| | | BN | $X^3\Pi$ | 2.05171 | 2.00636 | 2.00510 | 2.00289 | 2.00644 | 2.00383 | 2.00361 | 2.00340 |
| | | BO | $X^2\Sigma^+$ | 0.80067 | 0.76145 | 0.75971 | 0.75571 | 0.76350 | 0.75698 | 0.75704 | 0.75832 |
| | | CH | $X^2\Pi_r$ | 1.10075 | 0.75579 | 0.75551 | 0.75270 | 0.75428 | 0.75326 | 0.75279 | 0.75210 |
| | | $C_2^-$ | $X^2\Sigma_g^+$ | 0.75627 | 0.75579 | 0.75337 | 0.75332 | 0.75519 | 0.75544 | 0.76265 | 0.75835 |
| | | CN | $X^2\Sigma^+$ | 1.15755 | 0.76257 | 0.75580 | 0.75447 | 0.76131 | 0.75958 | 0.76000 | 0.76049 |
| | | $CO^+$ | $X^2\Sigma^+$ | 0.96970 | 0.76730 | 0.76261 | 0.75964 | 0.77442 | 0.76532 | 0.76466 | 0.76630 |
| | | CF | $X^2\Pi_r$ | 0.76275 | 0.75627 | 0.75584 | 0.75299 | 0.75435 | 0.75370 | 0.75333 | 0.75220 |
| | | NH | $X^3\Sigma^-$ | 2.01660 | 2.01005 | 2.00985 | 2.00481 | 2.01010 | 2.00706 | 2.00562 | 2.00603 |
| | | $N_2^+$ | $X^2\Sigma_g^+$ | 1.23889 | 0.75334 | 0.75207 | 0.75241 | 0.75417 | 0.75392 | 0.75423 | 0.75330 |
| | | NO | $X^2\Pi_r$ | 0.79621 | 0.75407 | 0.75343 | 0.75215 | 0.75368 | 0.75347 | 0.75324 | 0.75279 |
| | | NF | $X^3\Sigma^-$ | 2.02283 | 2.01047 | 2.00989 | 2.00507 | 2.00948 | 2.00795 | 2.00687 | 2.00626 |
| | | OH | $X^2\Pi_i$ | 0.75710 | 0.75446 | 0.75442 | 0.75224 | 0.75419 | 0.75299 | 0.75252 | 0.75279 |
| | | $HO^+$ | $X^3\Sigma^-$ | 2.01414 | 2.00868 | 2.00858 | 2.00419 | 2.00758 | 2.00594 | 2.00511 | 2.00583 |
| | | $O_2$ | $X^3\Sigma_g^-$ | 2.04908 | 2.00962 | 2.00751 | 2.00526 | 2.01025 | 2.00981 | 2.00954 | 2.00857 |
| | | $O_2^+$ | $X^2\Pi_g$ | 1.12597 | 0.75272 | 0.75229 | 0.75154 | 0.75292 | 0.75263 | 0.75259 | 0.75221 |
| | | $O_2^-$ | $X^2\Pi_{g,i}$ | 0.79527 | 0.75617 | 0.75395 | 0.75412 | 0.75787 | 0.75739 | 0.75710 | 0.75631 |
| | | OF | $X^2\Pi$ | 0.77257 | 0.75447 | 0.75390 | 0.75224 | 0.75436 | 0.75378 | 0.75348 | 0.75376 |
| | | $HF^+$ | $X^2\Pi_i$ | 0.75515 | 0.75336 | 0.75334 | 0.75169 | 0.75306 | 0.75219 | 0.75191 | 0.75209 |
| | | $F_2^+$ | $X^2\Pi_{g,i}$ | 0.82975 | 0.75265 | 0.75193 | 0.75152 | 0.75314 | 0.75303 | 0.75308 | 0.75292 |
| | | $F_2^-$ | $X^2\Sigma_u^+$ | 0.77276 | 0.75746 | 0.75533 | 0.75283 | 0.75568 | 0.75597 | 0.75578 | 0.75599 |
| | Row 2–Row 3 | Dimer | State | CCSD(T): UHF | CCSD(T): $\kappa$-OOMP2 | CCSD(T): OOMP2 | CCSD(T): BLYP | CCSD(T): B97M-rV | CCSD(T): B97 | CCSD(T): $\omega$B97X-V | CCSD(T): $\omega$B97M-V |
| | | NaO | $X^2\Pi$ | 0.76211 | 0.75797 | 0.75866 | 0.75946 | 0.76283 | 0.75888 | 0.75546 | 0.75688 |
| | | MgH | $X^2\Sigma^+$ | 0.75985 | 0.75613 | 0.75575 | 0.75320 | 0.75128 | 0.75330 | 0.75516 | 0.75388 |
| | | MgF | $X^2\Sigma^+$ | 0.75036 | 0.75048 | 0.75057 | 0.75025 | 0.75076 | 0.75062 | 0.75052 | 0.75049 |
| | | $AlH^+$ | $X^2\Sigma^+$ | 0.77723 | 0.76616 | 0.76425 | 0.75539 | 0.75413 | 0.75545 | 0.75903 | 0.75678 |
| | | SiH | $X^2\Pi_r$ | 0.79747 | 0.76132 | 0.75871 | 0.75404 | 0.75455 | 0.75485 | 0.75548 | 0.75211 |
| | | SiF | $X^2\Pi_r$ | 0.77677 | 0.76186 | 0.75908 | 0.75400 | 0.75480 | 0.75510 | 0.75597 | 0.75174 |
| | | PH | $X^3\Sigma^-$ | 2.02909 | 2.01225 | 2.01010 | 2.00492 | 2.00850 | 2.00709 | 2.00641 | 2.00395 |
| | | $PH^+$ | $X^2\Pi_r$ | 0.79438 | 0.75888 | 0.75781 | 0.75364 | 0.75465 | 0.75448 | 0.75437 | 0.75231 |

| | | | | | | | | | |
|---|---|---|---|---|---|---|---|---|---|
| | $PH^-$ | $X^2\Pi_i$ | 0.77186 | 0.76106 | 0.75950 | 0.75478 | 0.75708 | 0.75612 | 0.75523 | 0.75394 |
| | CP | $X^2\Sigma^+$ | 1.61297 | 0.82118 | 0.76087 | 0.76599 | 0.80531 | 0.78991 | 0.80446 | 0.79607 |
| | PO | $X^2\Pi_r$ | 0.77298 | 0.75758 | 0.75572 | 0.75301 | 0.75418 | 0.75438 | 0.75529 | 0.75258 |
| | $PO^-$ | $X^3\Sigma^-$ | 2.04447 | 2.00989 | 2.00729 | 2.00468 | 2.00812 | 2.00860 | 2.01013 | 2.00607 |
| | PF | $X^3\Sigma^-$ | 2.03511 | 2.01047 | 2.00788 | 2.00410 | 2.00876 | 2.00662 | 2.00654 | 2.00285 |
| | $PF^+$ | $X^2\Pi_r$ | 0.77166 | 0.75909 | 0.75772 | 0.75350 | 0.75552 | 0.75464 | 0.75478 | 0.75208 |
| | HS | $X^2\Pi_i$ | 0.76481 | 0.75738 | 0.75666 | 0.75337 | 0.75530 | 0.75420 | 0.75383 | 0.75266 |
| | BS | $X^2\Sigma^+$ | 0.85482 | 0.77318 | 0.76520 | 0.75858 | 0.77086 | 0.76235 | 0.76101 | 0.76416 |
| | $CS^+$ | $X^2\Sigma^+$ | 1.47259 | 0.80770 | 0.76914 | 0.77031 | 0.80860 | 0.79111 | 0.79583 | 0.79312 |
| | NS | $X^2\Pi_r$ | 1.18951 | 0.75758 | 0.75365 | 0.75377 | 0.75636 | 0.75751 | 0.75990 | 0.75736 |
| | SO | $X^3\Sigma^-$ | 2.05909 | 2.01059 | 2.00667 | 2.00507 | 2.00929 | 2.00982 | 2.01195 | 2.00851 |
| | $SO^+$ | $X^2\Pi_r$ | 1.18709 | 0.75583 | 0.75422 | 0.75259 | 0.75398 | 0.75413 | 0.75513 | 0.75304 |
| | $HCl^+$ | $X^2\Pi_i$ | 0.76226 | 0.75633 | 0.75598 | 0.75301 | 0.75489 | 0.75373 | 0.75332 | 0.75257 |
| | $LiCl^-$ | $X^2\Sigma^+$ | 0.75014 | 0.75016 | 0.75019 | 0.75008 | 0.75219 | 0.75038 | 0.75016 | 0.75018 |
| | BeCl | $X^2\Sigma^+$ | 0.75155 | 0.75140 | 0.75150 | 0.75094 | 0.75221 | 0.75078 | 0.75079 | 0.75078 |
| | CCl | $X^2\Pi$ | 0.76579 | 0.75772 | 0.75656 | 0.75355 | 0.75543 | 0.75493 | 0.75486 | 0.75405 |
| | NCl | $X^3\Sigma^-$ | 2.03589 | 2.01532 | 2.01178 | 2.00654 | 2.01180 | 2.01122 | 2.01189 | 2.01037 |
| | OCl | $X^2\Pi_i$ | 0.77010 | 0.75664 | 0.75405 | 0.75289 | 0.75543 | 0.75536 | 0.75629 | 0.75521 |
| | $FCl^+$ | $X^2\Pi$ | 0.76463 | 0.75541 | 0.75456 | 0.75221 | 0.75387 | 0.75348 | 0.75381 | 0.75267 |
| Row 3–Row 3 | Dimer | State | CCSD(T): UHF | CCSD(T): $\kappa$-OOMP2 | CCSD(T): OOMP2 | CCSD(T): BLYP | CCSD(T): B97M-rV | CCSD(T): B97 | CCSD(T): $\omega$B97X-V | CCSD(T): $\omega$B97M-V |
| | MgCl | $X^2\Sigma^+$ | 0.75092 | 0.75085 | 0.75093 | 0.75045 | 0.75059 | 0.75084 | 0.75094 | 0.75082 |
| | AlS | $X^2\Sigma^+$ | 0.77492 | 0.76188 | 0.75923 | 0.75355 | 0.75466 | 0.75498 | 0.75917 | 0.75552 |
| | $Si_2$ | $X^3\Sigma_g^-$ | 2.01897 | 2.00946 | 2.00560 | 2.00441 | 2.00890 | 2.00554 | 2.00422 | 2.00332 |
| | SiCl | $X^2\Pi_r$ | 0.77631 | 0.76144 | 0.75850 | 0.75402 | 0.75541 | 0.75517 | 0.75601 | 0.75208 |
| | $P_2^+$ | $X^2\Pi_u$ | 1.16866 | 0.75476 | 0.75651 | 0.75262 | 0.75510 | 0.75289 | 0.75237 | 0.75166 |
| | PS | $X^2\Pi_r$ | 1.05380 | 0.76119 | 0.75590 | 0.75340 | 0.75496 | 0.75557 | 0.75791 | 0.75445 |
| | $S_2$ | $X^3\Sigma_g^-$ | 2.06163 | 2.01837 | 2.00876 | 2.00494 | 2.00775 | 2.00936 | 2.01559 | 2.00936 |
| | $S_2^+$ | $X^2\Pi_{g,r}$ | 1.23007 | 0.75862 | 0.75431 | 0.75285 | 0.75386 | 0.75457 | 0.75747 | 0.75392 |

Table S9: Mean-field $\langle S^2 \rangle$ values for the reference methods at the CCSD minimum energy points used in the fitting procedure.

| Closed-shell | | Dimer | State | CCSD: UHF | CCSD: $\kappa$-OOMP2 | CCSD: OOMP2 | CCSD: BLYP | CCSD: B97M-rV | CCSD: B97 | CCSD: $\omega$B97X-V | CCSD: $\omega$B97M-V |
|---|---|---|---|---|---|---|---|---|---|---|---|
| | Row 2–Row 2 | | | | | | | | | | |
| | | LiH | $X^1\Sigma^+$ | 0.00000 | 0.00000 | 0.00000 | 0.00000 | 0.00000 | 0.00000 | 0.00000 | 0.00000 |
| | | $Li_2$ | $X^1\Sigma_g^+$ | 0.31690 | 0.00000 | 0.00000 | 0.00000 | 0.01065 | 0.00000 | 0.00000 | 0.00000 |
| | | LiF | $X^1\Sigma^+$ | 0.00000 | 0.00000 | 0.00000 | 0.00000 | 0.00000 | 0.00000 | 0.00000 | 0.00000 |
| | | $BeH^+$ | $X^1\Sigma^+$ | 0.00000 | 0.00000 | 0.00000 | 0.00000 | 0.00000 | 0.00000 | 0.00000 | 0.00000 |
| | | BeO | $X^1\Sigma^+$ | 0.00000 | 0.00000 | 0.00000 | 0.00000 | 0.00000 | 0.00000 | 0.00000 | 0.00000 |
| | | BH | $X^1\Sigma^+$ | 0.47646 | 0.04871 | 0.00000 | 0.03506 | 0.00000 | 0.00000 | 0.00000 | 0.00000 |
| | | BF | $X^1\Sigma^+$ | 0.00000 | 0.00000 | 0.00000 | 0.00000 | 0.00000 | 0.00000 | 0.00000 | 0.00000 |
| | | $C_2$ | $X^1\Sigma_g^+$ | 1.62372 | 0.90291 | 0.00000 | 0.92892 | 1.00478 | 1.00057 | 1.05327 | 1.02472 |
| | | CO | $X^1\Sigma^+$ | 0.00000 | 0.00000 | 0.00000 | 0.00000 | 0.00000 | 0.00000 | 0.00000 | 0.00000 |
| | | $N_2$ | $X^1\Sigma_g^+$ | 0.00000 | 0.00000 | 0.00000 | 0.00000 | 0.00000 | 0.00000 | 0.00000 | 0.00000 |
| | | $NO^+$ | $X^1\Sigma^+$ | 0.00000 | 0.00000 | 0.00000 | 0.00000 | 0.00000 | 0.00000 | 0.00000 | 0.00000 |
| | | $OH^-$ | $X^1\Sigma^+$ | 0.00000 | 0.00000 | 0.00000 | 0.00000 | 0.00000 | 0.00000 | 0.00000 | 0.00000 |
| | | HF | $X^1\Sigma^+$ | 0.00000 | 0.00000 | 0.00000 | 0.00000 | 0.00000 | 0.00000 | 0.00000 | 0.00000 |
| | | $F_2$ | $X^1\Sigma_g^+$ | 0.21545 | 0.00000 | 0.00000 | 0.00000 | 0.00000 | 0.00000 | 0.00000 | 0.00000 |
| | Row 2–Row 3 | Dimer | State | CCSD: UHF | CCSD: $\kappa$-OOMP2 | CCSD: OOMP2 | CCSD: BLYP | CCSD: B97M-rV | CCSD: B97 | CCSD: $\omega$B97X-V | CCSD: $\omega$B97M-V |
| | | NaH | $X^1\Sigma^+$ | 0.00000 | 0.00000 | 0.00000 | 0.00000 | 0.00000 | 0.00000 | 0.00000 | 0.00000 |
| | | NaLi | $X^1\Sigma^+$ | 0.32702 | 0.03641 | 0.00000 | 0.00000 | 0.00000 | 0.00000 | 0.00000 | 0.00000 |
| | | NaF | $X^1\Sigma^+$ | 0.00000 | 0.00000 | 0.00000 | 0.00000 | 0.00000 | 0.00000 | 0.00000 | 0.00000 |
| | | $MgH^+$ | $X^1\Sigma^+$ | 0.00000 | 0.00000 | 0.00000 | 0.00000 | 0.00000 | 0.00000 | 0.00000 | 0.00000 |
| | | AlH | $X^1\Sigma^+$ | 0.17105 | 0.00000 | 0.00000 | 0.00000 | 0.00000 | 0.00000 | 0.00000 | 0.00000 |
| | | AlF | $X^1\Sigma^+$ | 0.00000 | 0.00000 | 0.00000 | 0.00000 | 0.00000 | 0.00000 | 0.00000 | 0.00000 |
| | | $SiH^+$ | $X^1\Sigma^+$ | 0.06997 | 0.00000 | 0.00000 | 0.00000 | 0.00000 | 0.00000 | 0.00000 | 0.00000 |
| | | SiO | $X^1\Sigma^+$ | 0.00000 | 0.00000 | 0.00000 | 0.00000 | 0.00000 | 0.00000 | 0.00000 | 0.00000 |
| | | PN | $X^1\Sigma^+$ | 0.65868 | 0.00000 | 0.00000 | 0.00000 | 0.00000 | 0.00000 | 0.00000 | 0.00000 |
| | | BeS | $X^1\Sigma^+$ | 1.01646 | 0.00000 | 0.00000 | 0.00000 | 0.00000 | 0.00000 | 0.00000 | 0.00000 |
| | | CS | $X^1\Sigma^+$ | 0.00000 | 0.00000 | 0.00000 | 0.00000 | 0.00000 | 0.00000 | 0.00000 | 0.00000 |
| | | $NS^+$ | $X^1\Sigma^+$ | 0.64038 | 0.00000 | 0.00000 | 0.00000 | 0.00000 | 0.00000 | 0.00000 | 0.00000 |
| | | HCl | $X^1\Sigma^+$ | 0.00000 | 0.00000 | 0.00000 | 0.00000 | 0.00000 | 0.00000 | 0.00000 | 0.00000 |
| | | LiCl | $X^1\Sigma^+$ | 0.00000 | 0.00000 | 0.00000 | 0.00000 | 0.00000 | 0.00000 | 0.00000 | 0.00000 |
| | | BCl | $X^1\Sigma^+$ | 0.17638 | 0.00000 | 0.00000 | 0.00000 | 0.00000 | 0.00000 | 0.00000 | 0.00000 |
| | | $CCl^+$ | $X^1\Sigma^+$ | 0.00000 | 0.00000 | 0.00000 | 0.00000 | 0.00000 | 0.00000 | 0.00000 | 0.00000 |
| | | ClF | $X^1\Sigma^+$ | 0.00000 | 0.00000 | 0.00000 | 0.00000 | 0.00000 | 0.00000 | 0.00000 | 0.00000 |
| | Row 3–Row 3 | Dimer | State | CCSD: UHF | CCSD: $\kappa$-OOMP2 | CCSD: OOMP2 | CCSD: BLYP | CCSD: B97M-rV | CCSD: B97 | CCSD: $\omega$B97X-V | CCSD: $\omega$B97M-V |
| | | NaCl | $X^1\Sigma^+$ | 0.00000 | 0.00000 | 0.00000 | 0.00000 | 0.00000 | 0.00000 | 0.00000 | 0.00000 |

| | | | | | | | | | | | |
|---|---|---|---|---|---|---|---|---|---|---|---|
| | | AlCl | $X^1\Sigma^+$ | 0.00000 | 0.00000 | 0.00000 | 0.00000 | 0.00000 | 0.00000 | 0.00000 | 0.00000 |
| | | SiS | $X^1\Sigma^+$ | 0.00000 | 0.00000 | 0.00000 | 0.00000 | 0.00000 | 0.00000 | 0.00000 | 0.00000 |
| | | $P_2$ | $X^1\Sigma_g^+$ | 0.60962 | 0.00000 | 0.00000 | 0.00000 | 0.00000 | 0.00000 | 0.00000 | 0.00000 |
| | | $Cl_2$ | $X^1\Sigma_g^+$ | 0.00000 | 0.00000 | 0.00000 | 0.00000 | 0.00000 | 0.00000 | 0.00000 | 0.00000 |
| Open-shell | Row 2–Row 2 | Dimer | State | CCSD: UHF | CCSD: $\kappa$-OOMP2 | CCSD: OOMP2 | CCSD: BLYP | CCSD: B97M-rV | CCSD: B97 | CCSD: $\omega$B97X-V | CCSD: $\omega$B97M-V |
| | | LiO | $X^2\Pi_i$ | 0.75966 | 0.75599 | 0.75607 | 0.75366 | 0.75613 | 0.75475 | 0.75369 | 0.75435 |
| | | BeH | $X^2\Sigma^+$ | 0.75204 | 0.75136 | 0.75144 | 0.75100 | 0.75042 | 0.75068 | 0.75107 | 0.75052 |
| | | BeF | $X^2\Sigma^+$ | 0.75084 | 0.75096 | 0.75103 | 0.75058 | 0.75212 | 0.75065 | 0.75065 | 0.75050 |
| | | $B_2$ | $X^3\Sigma_g^-$ | 2.91265 | 2.82216 | 2.00956 | 2.40515 | 2.50830 | 2.54165 | 2.69514 | 2.61548 |
| | | BN | $X^3\Pi$ | 2.04561 | 2.00633 | 2.00510 | 2.00286 | 2.00650 | 2.00377 | 2.00355 | 2.00337 |
| | | BO | $X^2\Sigma^+$ | 0.79782 | 0.76122 | 0.75955 | 0.75559 | 0.76313 | 0.75683 | 0.75689 | 0.75813 |
| | | CH | $X^2\Pi_r$ | 1.10075 | 0.75579 | 0.75551 | 0.75270 | 0.75428 | 0.75326 | 0.75279 | 0.75210 |
| | | $C_2^-$ | $X^2\Sigma_g^+$ | 0.75628 | 0.75577 | 0.75338 | 0.75331 | 0.75516 | 0.75534 | 0.76049 | 0.75748 |
| | | CN | $X^2\Sigma^+$ | 1.11881 | 0.76253 | 0.75590 | 0.75441 | 0.76117 | 0.75942 | 0.75973 | 0.76030 |
| | | $CO^+$ | $X^2\Sigma^+$ | 0.95712 | 0.76676 | 0.76253 | 0.75924 | 0.77298 | 0.76444 | 0.76379 | 0.76536 |
| | | CF | $X^2\Pi_r$ | 0.76271 | 0.75624 | 0.75582 | 0.75297 | 0.75432 | 0.75368 | 0.75331 | 0.75218 |
| | | NH | $X^3\Sigma^-$ | 2.01660 | 2.01005 | 2.00985 | 2.00481 | 2.01010 | 2.00706 | 2.00562 | 2.00603 |
| | | $N_2^+$ | $X^2\Sigma_g^+$ | 1.19138 | 0.75333 | 0.75212 | 0.75232 | 0.75406 | 0.75377 | 0.75416 | 0.75316 |
| | | NO | $X^2\Pi_r$ | 0.78638 | 0.75402 | 0.75344 | 0.75209 | 0.75356 | 0.75333 | 0.75311 | 0.75265 |
| | | NF | $X^3\Sigma^-$ | 2.02281 | 2.01045 | 2.00989 | 2.00505 | 2.00944 | 2.00791 | 2.00683 | 2.00616 |
| | | OH | $X^2\Pi_i$ | 0.75710 | 0.75446 | 0.75442 | 0.75224 | 0.75419 | 0.75299 | 0.75252 | 0.75279 |
| | | $HO^+$ | $X^3\Sigma^-$ | 2.01414 | 2.00868 | 2.00858 | 2.00419 | 2.00758 | 2.00594 | 2.00511 | 2.00583 |
| | | $O_2$ | $X^3\Sigma_g^-$ | 2.04740 | 2.00967 | 2.00772 | 2.00516 | 2.01004 | 2.00958 | 2.00927 | 2.00834 |
| | | $O_2^+$ | $X^2\Pi_g$ | 1.08640 | 0.75274 | 0.75233 | 0.75153 | 0.75289 | 0.75259 | 0.75255 | 0.75217 |
| | | $O_2^-$ | $X^2\Pi_{g,i}$ | 0.79295 | 0.75622 | 0.75417 | 0.75405 | 0.75767 | 0.75718 | 0.75684 | 0.75610 |
| | | OF | $X^2\Pi$ | 0.76696 | 0.75440 | 0.75391 | 0.75219 | 0.75425 | 0.75364 | 0.75335 | 0.75353 |
| | | $HF^+$ | $X^2\Pi_i$ | 0.75510 | 0.75334 | 0.75332 | 0.75168 | 0.75304 | 0.75218 | 0.75189 | 0.75207 |
| | | $F_2^+$ | $X^2\Pi_{g,i}$ | 0.79656 | 0.75276 | 0.75213 | 0.75150 | 0.75312 | 0.75298 | 0.75302 | 0.75285 |
| | | $F_2^-$ | $X^2\Sigma_u^+$ | 0.77581 | 0.75739 | 0.75531 | 0.75281 | 0.75565 | 0.75591 | 0.75571 | 0.75592 |
| | Row 2–Row 3 | Dimer | State | CCSD: UHF | CCSD: $\kappa$-OOMP2 | CCSD: OOMP2 | CCSD: BLYP | CCSD: B97M-rV | CCSD: B97 | CCSD: $\omega$B97X-V | CCSD: $\omega$B97M-V |
| | | NaO | $X^2\Pi$ | 0.76205 | 0.75794 | 0.75863 | 0.75938 | 0.76271 | 0.75882 | 0.75544 | 0.75684 |
| | | MgH | $X^2\Sigma^+$ | 0.75985 | 0.75613 | 0.75575 | 0.75320 | 0.75128 | 0.75330 | 0.75516 | 0.75388 |
| | | MgF | $X^2\Sigma^+$ | 0.75036 | 0.75048 | 0.75057 | 0.75024 | 0.75076 | 0.75061 | 0.75051 | 0.75048 |
| | | $AlH^+$ | $X^2\Sigma^+$ | 0.77723 | 0.76584 | 0.76400 | 0.75531 | 0.75403 | 0.75536 | 0.75887 | 0.75666 |
| | | SiH | $X^2\Pi_r$ | 0.79747 | 0.76132 | 0.75871 | 0.75404 | 0.75455 | 0.75485 | 0.75548 | 0.75211 |
| | | SiF | $X^2\Pi_r$ | 0.77677 | 0.76186 | 0.75908 | 0.75400 | 0.75479 | 0.75510 | 0.75597 | 0.75174 |
| | | PH | $X^3\Sigma^-$ | 2.02913 | 2.01224 | 2.01007 | 2.00492 | 2.00848 | 2.00709 | 2.00641 | 2.00394 |
| | | $PH^+$ | $X^2\Pi_r$ | 0.79445 | 0.75887 | 0.75780 | 0.75364 | 0.75464 | 0.75447 | 0.75437 | 0.75231 |

| | | | | | | | | | | |
|---|---|---|---|---|---|---|---|---|---|---|
| | $PH^-$ | $X^2\Pi_i$ | 0.77189 | 0.76106 | 0.75949 | 0.75478 | 0.75707 | 0.75612 | 0.75523 | 0.75394 |
| | CP | $X^2\Sigma^+$ | 1.59712 | 0.81614 | 0.76132 | 0.76525 | 0.80179 | 0.78701 | 0.79906 | 0.79240 |
| | PO | $X^2\Pi_r$ | 0.77267 | 0.75758 | 0.75576 | 0.75300 | 0.75413 | 0.75434 | 0.75522 | 0.75252 |
| | $PO^-$ | $X^3\Sigma^-$ | 2.04349 | 2.00978 | 2.00720 | 2.00460 | 2.00799 | 2.00841 | 2.00993 | 2.00591 |
| | PF | $X^3\Sigma^-$ | 2.03511 | 2.01048 | 2.00788 | 2.00411 | 2.00875 | 2.00663 | 2.00655 | 2.00284 |
| | $PF^+$ | $X^2\Pi_r$ | 0.77166 | 0.75910 | 0.75772 | 0.75350 | 0.75550 | 0.75464 | 0.75478 | 0.75207 |
| | HS | $X^2\Pi_i$ | 0.76481 | 0.75737 | 0.75664 | 0.75337 | 0.75530 | 0.75420 | 0.75383 | 0.75266 |
| | BS | $X^2\Sigma^+$ | 0.85146 | 0.77281 | 0.76503 | 0.75844 | 0.77046 | 0.76215 | 0.76083 | 0.76394 |
| | $CS^+$ | $X^2\Sigma^+$ | 1.44109 | 0.80436 | 0.76927 | 0.76925 | 0.80472 | 0.78827 | 0.79187 | 0.78999 |
| | NS | $X^2\Pi_r$ | 1.16463 | 0.75742 | 0.75373 | 0.75364 | 0.75599 | 0.75702 | 0.75917 | 0.75672 |
| | SO | $X^3\Sigma^-$ | 2.05772 | 2.01052 | 2.00679 | 2.00498 | 2.00905 | 2.00958 | 2.01162 | 2.00823 |
| | $SO^+$ | $X^2\Pi_r$ | 1.12991 | 0.75587 | 0.75431 | 0.75259 | 0.75396 | 0.75408 | 0.75502 | 0.75297 |
| | $HCl^+$ | $X^2\Pi_i$ | 0.76225 | 0.75631 | 0.75597 | 0.75300 | 0.75488 | 0.75372 | 0.75332 | 0.75257 |
| | $LiCl^-$ | $X^2\Sigma^+$ | 0.75014 | 0.75016 | 0.75019 | 0.75008 | 0.75219 | 0.75038 | 0.75016 | 0.75018 |
| | BeCl | $X^2\Sigma^+$ | 0.75155 | 0.75140 | 0.75150 | 0.75094 | 0.75221 | 0.75078 | 0.75079 | 0.75078 |
| | CCl | $X^2\Pi$ | 0.76583 | 0.75771 | 0.75655 | 0.75354 | 0.75541 | 0.75492 | 0.75486 | 0.75403 |
| | NCl | $X^3\Sigma^-$ | 2.03586 | 2.01531 | 2.01178 | 2.00653 | 2.01177 | 2.01119 | 2.01188 | 2.01031 |
| | OCl | $X^2\Pi_i$ | 0.77006 | 0.75662 | 0.75412 | 0.75287 | 0.75540 | 0.75531 | 0.75626 | 0.75515 |
| | $FCl^+$ | $X^2\Pi$ | 0.76481 | 0.75542 | 0.75461 | 0.75222 | 0.75388 | 0.75348 | 0.75380 | 0.75265 |
| Row 3–Row 3 | Dimer | State | CCSD: UHF | CCSD: $\kappa$-OOMP2 | CCSD: OOMP2 | CCSD: BLYP | CCSD: B97M-rV | CCSD: B97 | CCSD: $\omega$B97X-V | CCSD: $\omega$B97M-V |
| | MgCl | $X^2\Sigma^+$ | 0.75092 | 0.75084 | 0.75093 | 0.75045 | 0.75059 | 0.75083 | 0.75093 | 0.75081 |
| | AlS | $X^2\Sigma^+$ | 0.77348 | 0.76156 | 0.75911 | 0.75350 | 0.75457 | 0.75487 | 0.75886 | 0.75537 |
| | $Si_2$ | $X^3\Sigma_g^-$ | 2.01899 | 2.00949 | 2.00565 | 2.00442 | 2.00891 | 2.00555 | 2.00423 | 2.00335 |
| | SiCl | $X^2\Pi_r$ | 0.77634 | 0.76144 | 0.75850 | 0.75402 | 0.75540 | 0.75517 | 0.75602 | 0.75208 |
| | ${P_2}^+$ | $X^2\Pi_u$ | 1.13370 | 0.75477 | 0.75663 | 0.75262 | 0.75508 | 0.75289 | 0.75237 | 0.75167 |
| | PS | $X^2\Pi_r$ | 1.02029 | 0.76093 | 0.75592 | 0.75338 | 0.75484 | 0.75545 | 0.75780 | 0.75429 |
| | $S_2$ | $X^3\Sigma_g^-$ | 2.06113 | 2.01829 | 2.00891 | 2.00493 | 2.00775 | 2.00931 | 2.01545 | 2.00924 |
| | ${S_2}^+$ | $X^2\Pi_{g,r}$ | 1.20499 | 0.75864 | 0.75444 | 0.75286 | 0.75388 | 0.75456 | 0.75743 | 0.75388 |

# 4 CCSD data

Table S10: Experimental vibrational frequencies and errors in the corrected vibrational frequencies for the closed-shell species are presented in for the CCSD methods utilizing different molecular orbitals. Root mean square deviations, mean signed deviations, minimum deviations, and maximum deviations for the set of species and subsets are also presented.

| Row 2–Row 2 | Dimer | State | Expt. | Δ(CCSD: UHF) | Δ(CCSD: κ-OOMP2) | Δ(CCSD: OOMP2) | Δ(CCSD: BLYP) | Δ(CCSD: B97M-rV) | Δ(CCSD: B97) | Δ(CCSD: ωB97X-V) | Δ(CCSD: ωB97M-V) |
|---|---|---|---|---|---|---|---|---|---|---|---|
| | LiH | $X^1\Sigma^+$ | 1405.49805[a] | -4.95 | -5.93 | -5.25 | -3.96 | -6.91 | -7.45 | -4.46 | -5.49 |
| | $Li_2$ | $X^1\Sigma_g^+$ | 351.4066[a] | -4.86 | -10.16 | -3.10 | -4.03 | -1.75 | -3.36 | -26.61 | -4.36 |
| | LiF | $X^1\Sigma^+$ | 910.57272[a] | 4.40 | 6.56 | 7.19 | 7.72 | 6.80 | 6.80 | 6.57 | 6.45 |
| | $BeH^+$ | $X^1\Sigma^+$ | 2221.7[b] | -10.75 | -10.66 | -8.80 | -10.75 | -16.01 | -8.7694 | -13.26 | -8.97 |
| | BeO | $X^1\Sigma^+$ | 1487.32[b] | 75.94 | 88.76 | 93.78 | 91.43 | 89.12 | 90.2704 | 86.98 | 87.69 |
| | BH | $X^1\Sigma^+$ | 2366.7296[a] | 12.83 | 8.70 | 12.76 | 15.81 | 8.90 | 14.66 | 11.03 | 10.41 |
| | BF | $X^1\Sigma^+$ | 1402.15865[a] | 9.33 | 15.33 | 16.66 | 18.28 | 16.10 | 16.28 | 15.51 | 15.68 |
| | $C_2$ | $X^1\Sigma_g^+$ | 1855.0663[a] | 96.46 | 85.08 | 78.07 | -385.19 | -366.32 | -362.08 | -340.93 | -356.99 |
| | CO | $X^1\Sigma^+$ | 2169.75589[a] | 55.68 | 70.60 | 73.72 | 72.33 | 68.78 | 68.93 | 67.27 | 67.34 |
| | $N_2$ | $X^1\Sigma_g^+$ | 2358.57[a] | 76.36 | 88.42 | 91.17 | 89.58 | 86.00 | 86.76 | 84.80 | 84.93 |
| | $NO^+$ | $X^1\Sigma^+$ | 2376.72[a] | 103.61 | 123.66 | 127.13 | 123.61 | 119.47 | 118.90 | 117.38 | 117.44 |
| | $OH^-$ | $X^1\Sigma^+$ | 3735.2[c] | 52.95 | 69.59 | 76.05 | 69.57 | 65.42 | 65.63 | 64.56 | 64.61 |
| | HF | $X^1\Sigma^+$ | 4138.385[a] | 39.17 | 48.26 | 49.86 | 49.91 | 46.21 | 48.53 | 46.91 | 46.61 |
| | $F_2$ | $X^1\Sigma_g^+$ | 916.929[d] | 170.29 | 104.70 | 107.50 | 104.74 | 103.50 | 103.32 | 102.90 | 102.84 |
| | RMSD | | | 69.95 | 66.52 | 68.26 | 120.82 | 115.37 | 114.54 | 109.40 | 112.80 |
| | MSD | | | 48.32 | 48.78 | 51.20 | 17.07 | 15.67 | 17.03 | 15.62 | 16.30 |
| | MIN | | | -10.75 | -10.66 | -8.80 | -385.19 | -366.32 | -362.08 | -340.93 | -356.99 |
| | MAX | | | 170.29 | 123.66 | 127.13 | 123.61 | 119.47 | 118.90 | 117.38 | 117.44 |
| Row 2–Row 3 | Dimer | State | Expt. | Δ(CCSD: UHF) | Δ(CCSD: κ-OOMP2) | Δ(CCSD: OOMP2) | Δ(CCSD: BLYP) | Δ(CCSD: B97M-rV) | Δ(CCSD: B97) | Δ(CCSD: ωB97X-V) | Δ(CCSD: ωB97M-V) |
| | NaH | $X^1\Sigma^+$ | 1171.968[a] | -8.37 | -8.55 | -8.45 | -10.03 | -8.69 | -9.60 | -9.63 | -9.82 |
| | NaLi | $X^1\Sigma^+$ | 256.5412[a] | 2.01 | 2.11 | -2.86 | -0.47 | -0.59 | -15.03 | -3.63 | -2.49 |
| | NaF | $X^1\Sigma^+$ | 535.65805[a] | 0.17 | 1.57 | 1.93 | 2.13 | 1.72 | 1.52 | 1.57 | 1.63 |
| | $MgH^+$ | $X^1\Sigma^+$ | 1699.1[b] | -0.10 | -0.17 | 1.38 | -1.86 | -3.39 | 0.23 | -1.82 | -3.41 |
| | AlH | $X^1\Sigma^+$ | 1682.37474[a] | -7.02 | -2.63 | -6.91 | -3.94 | -8.11 | -1.94 | -2.19 | -4.07 |
| | AlF | $X^1\Sigma^+$ | 802.32447[a] | 2.01 | 4.73 | 5.55 | 6.33 | 5.17 | 5.24 | 4.87 | 4.99 |
| | $SiH^+$ | $X^1\Sigma^+$ | 2157.17[a] | 8.25 | 12.28 | 12.44 | 14.13 | 14.30 | 13.86 | 8.73 | 12.63 |
| | SiO | $X^1\Sigma^+$ | 1241.54388[a] | 43.96 | 53.88 | 59.60 | 56.14 | 54.35 | 53.99 | 51.85 | 51.92 |
| | PN | $X^1\Sigma^+$ | 1336.948[a] | 73.08 | 72.09 | 79.35 | 73.46 | 71.43 | 71.25 | 69.02 | 69.04 |
| | BeS | $X^1\Sigma^+$ | 997.94[a] | -234.21 | 27.17 | 30.29 | 30.00 | 28.94 | 28.73 | 26.82 | 26.97 |
| | CS | $X^1\Sigma^+$ | 1285.08[b] | 51.17 | 62.22 | 68.15 | 65.08 | 62.36 | 62.60 | 59.60 | 60.19 |
| | $NS^+$ | $X^1\Sigma^+$ | 1415[b] | 100.80 | 102.09 | 109.97 | 103.13 | 100.22 | 100.32 | 97.92 | 98.31 |
| | HCl | $X^1\Sigma^+$ | 2990.9248[a] | 43.02 | 44.49 | 43.89 | 44.69 | 46.48 | 44.55 | 44.46 | 46.52 |
| | LiCl | $X^1\Sigma^+$ | 642.95453[a] | -3.92 | -3.82 | -3.91 | -3.63 | -3.61 | -3.68 | -4.01 | -3.62 |

| | | | | | | | | | | |
|---|---|---|---|---|---|---|---|---|---|---|
| | BCl | $X^1\Sigma^+$ | 840.29472[a] | 5.09 | 7.21 | 8.77 | 10.30 | 9.28 | 8.85 | 7.72 | 7.96 |
| | $CCl^+$ | $X^1\Sigma^+$ | 1175[b] | 44.47 | 58.67 | 66.11 | 63.50 | 60.07 | 60.05 | 56.25 | 57.15 |
| | ClF | $X^1\Sigma^+$ | 783.4534[a] | 28.96 | 32.27 | 33.38 | 32.36 | 31.19 | 31.30 | 31.19 | 31.16 |
| | RMSD | | | 68.52 | 41.95 | 45.59 | 43.30 | 42.05 | 42.01 | 40.38 | 40.78 |
| | MSD | | | 8.79 | 27.39 | 29.34 | 28.31 | 27.13 | 26.60 | 25.81 | 26.18 |
| | MIN | | | -234.21 | -8.55 | -8.45 | -10.03 | -8.69 | -15.03 | -9.63 | -9.82 |
| | MAX | | | 100.80 | 102.09 | 109.97 | 103.13 | 100.22 | 100.32 | 97.92 | 98.31 |
| Row 3–Row 3 | Dimer | State | Expt. | Δ(CCSD: UHF) | Δ(CCSD: κ-OOMP2) | Δ(CCSD: OOMP2) | Δ(CCSD: BLYP) | Δ(CCSD: B97M-rV) | Δ(CCSD: B97) | Δ(CCSD: ωB97X-V) | Δ(CCSD: ωB97M-V) |
| | NaCl | $X^1\Sigma^+$ | 364.6842[a] | -3.81 | -3.88 | -3.69 | -3.55 | -3.70 | -3.67 | -3.77 | -3.76 |
| | AlCl | $X^1\Sigma^+$ | 481.77466[a] | -4.67 | -4.48 | -4.13 | -3.65 | -4.00 | -3.98 | -4.33 | -4.30 |
| | SiS | $X^1\Sigma^+$ | 749.64559[a] | 21.34 | 24.75 | 28.00 | 27.66 | 26.51 | 26.39 | 24.47 | 24.83 |
| | $P_2$ | $X^1\Sigma_g^+$ | 780.77[a] | 45.20 | 39.47 | 42.93 | 41.59 | 40.53 | 40.57 | 38.80 | 38.96 |
| | $Cl_2$ | $X^1\Sigma_g^+$ | 559.751[a] | 7.82 | 8.43 | 8.85 | 9.01 | 8.74 | 8.56 | 8.46 | 8.46 |
| | RMSD | | | 22.79 | 21.34 | 23.39 | 22.81 | 22.15 | 22.11 | 21.02 | 21.16 |
| | MSD | | | 13.18 | 12.86 | 14.39 | 14.21 | 13.62 | 13.57 | 12.73 | 12.84 |
| | MIN | | | -4.67 | -4.48 | -4.13 | -3.65 | -4.00 | -3.98 | -4.33 | -4.30 |
| | MAX | | | 45.20 | 39.47 | 42.93 | 41.59 | 40.53 | 40.57 | 38.80 | 38.96 |
| Closed-shell | Dimer | State | Expt. | Δ(CCSD: UHF) | Δ(CCSD: κ-OOMP2) | Δ(CCSD: OOMP2) | Δ(CCSD: BLYP) | Δ(CCSD: B97M-rV) | Δ(CCSD: B97) | Δ(CCSD: ωB97X-V) | Δ(CCSD: ωB97M-V) |
| | RMSD | | | 64.75 | 51.14 | 53.57 | 81.45 | 77.97 | 77.48 | 74.07 | 76.13 |
| | MSD | | | 24.77 | 33.69 | 35.76 | 21.98 | 20.79 | 21.07 | 20.03 | 20.48 |
| | MIN | | | -234.21 | -10.66 | -8.80 | -385.19 | -366.32 | -362.08 | -340.93 | -356.99 |
| | MAX | | | 170.29 | 123.66 | 127.13 | 123.61 | 119.47 | 118.90 | 117.38 | 117.44 |

[a] From Ref. **?** .
[b] From Ref. **?** .
[c] From Ref. **?** .

Table S11: Experimental vibrational frequencies and errors in the corrected vibrational frequencies for the open-shell species are presented in for the CCSD methods utilizing different molecular orbitals. Root mean square deviations, mean signed deviations, minimum deviations, and maximum deviations for the set of species and subsets are presented.

| Row 2–Row 2 | Dimer | State | Expt. | Δ(CCSD:UHF) | Δ(CCSD:κ-OOMP2) | Δ(CCSD:OOMP2) | Δ(CCSD:BLYP) | Δ(CCSD:B97M-rV) | Δ(CCSD:B97) | Δ(CCSD:ωB97X-V) | Δ(CCSD:ωB97M-V) |
|---|---|---|---|---|---|---|---|---|---|---|---|
| | LiO | $X^2\Pi_i$ | 814.62[a] | 3.94 | 5.61 | 6.08 | 7.31 | 6.48 | 6.51 | 5.95 | 5.91 |
| | BeH | $X^2\Sigma^+$ | 2061.235[a] | 1.68 | 1.23 | 4.44 | 2.76 | 0.82 | 1.41 | 2.78 | 1.21 |
| | BeF | $X^2\Sigma^+$ | 1247.36[b] | 22.61 | 25.70 | 26.43 | 27.35 | 26.14 | 26.17 | 25.81 | 26.03 |
| | $B_2$ | $X^3\Sigma_g^-$ | 1051.3[b] | 44.59 | 40.38 | 3.78 | 35.49 | 33.05 | 31.27 | 32.03 | 32.73 |
| | BN | $X^3\Pi$ | 1514.6[b] | 64.98 | 68.38 | 71.04 | 68.20 | 66.68 | 65.12 | 64.42 | 66.43 |
| | BO | $X^2\Sigma^+$ | 1885.286[a] | 43.31 | 55.40 | 59.77 | 58.97 | 54.94 | 55.58 | 54.35 | 54.42 |
| | CH | $X^2\Pi_r$ | 2860.7508[a] | 14.37 | 22.42 | 20.91 | 23.07 | 22.30 | 20.99 | 20.73 | 22.84 |
| | $C_2^-$ | $X^2\Sigma_g^+$ | 1781.189[a] | -65.13 | 57.66 | 64.77 | 58.17 | 55.07 | 54.40 | 6.09 | 25.65 |
| | CN | $X^2\Sigma^+$ | 2068.648[a] | 103.60 | 78.37 | 81.29 | 76.63 | 75.27 | 74.70 | 73.98 | 75.70 |
| | $CO^+$ | $X^2\Sigma^+$ | 2214.127[a] | 91.85 | 112.67 | 119.04 | 113.90 | 105.88 | 107.95 | 106.78 | 107.09 |
| | CF | $X^2\Pi_r$ | 1307.93[a] | 28.27 | 39.55 | 42.36 | 43.55 | 40.34 | 40.11 | 38.60 | 38.82 |
| | NH | $X^3\Sigma^-$ | 3282.72[a] | 28.52 | 34.79 | 32.86 | 36.15 | 33.80 | 34.03 | 30.57 | 32.40 |
| | $N_2^+$ | $X^2\Sigma_g^+$ | 2207.0115[a] | 116.78 | 101.46 | 112.23 | 97.51 | 92.54 | 92.63 | 90.12 | 90.71 |
| | NO | $X^2\Pi_r$ | 1904.1346[a] | 89.82 | 104.51 | 108.95 | 105.22 | 100.93 | 101.24 | 99.29 | 99.51 |
| | NF | $X^3\Sigma^-$ | 1141.37[a] | 28.52 | 42.43 | 47.39 | 47.22 | 41.43 | 41.84 | 39.87 | 39.49 |
| | OH | $X^2\Pi_i$ | 3737.761[a] | 30.46 | 36.53 | 36.58 | 38.33 | 35.95 | 36.01 | 36.65 | 35.49 |
| | $OH^+$ | $X^3\Sigma^-$ | 3113.37[b] | 33.25 | 35.47 | 35.67 | 38.43 | 39.19 | 36.47 | 34.66 | 36.60 |
| | $O_2$ | $X^3\Sigma_g^-$ | 1580.161[a] | 81.40 | 99.60 | 104.70 | 99.11 | 95.69 | 95.12 | 93.78 | 93.88 |
| | $O_2^+$ | $X^2\Pi_g$ | 1905.892[a] | 133.11 | 150.65 | 156.65 | 148.73 | 144.25 | 144.04 | 142.11 | 142.24 |
| | $O_2^-$ | $X^2\Pi_{g,i}$ | 1090[b] | 102.15 | 119.79 | 127.46 | 118.74 | 116.16 | 115.49 | 114.22 | 114.17 |
| | OF | $X^2\Pi$ | 1053.0138[a] | 50.04 | 75.93 | 93.00 | 79.55 | 68.15 | 68.72 | 65.06 | 64.20 |
| | $HF^+$ | $X^2\Pi_i$ | 3090.5[b] | 57.35 | 59.59 | 59.35 | 66.31 | 60.95 | 62.06 | 61.75 | 61.82 |
| | $F_2^+$ | $X^2\Pi_{g,i}$ | 1091.5[d] | 153.52 | 152.75 | 161.40 | 150.43 | 148.16 | 147.68 | 146.35 | 145.97 |
| | $F_2^-$ | $X^2\Sigma_u^+$ | 510[b] | -24.34 | -49.85 | -47.22 | -49.21 | -50.23 | -50.31 | -50.52 | -50.67 |
| | RMSD | | | 71.63 | 77.25 | 81.44 | 77.39 | 74.18 | 74.08 | 72.10 | 72.54 |
| | MSD | | | 51.44 | 61.29 | 63.71 | 62.16 | 58.92 | 58.72 | 55.64 | 56.78 |
| | MIN | | | -65.13 | -49.85 | -47.22 | -49.21 | -50.23 | -50.31 | -50.52 | -50.67 |
| | MAX | | | 153.52 | 152.75 | 161.40 | 150.43 | 148.16 | 147.68 | 146.35 | 145.97 |
| Row 2–Row 3 | Dimer | State | Expt. | Δ(CCSD:UHF) | Δ(CCSD:κ-OOMP2) | Δ(CCSD:OOMP2) | Δ(CCSD:BLYP) | Δ(CCSD:B97M-rV) | Δ(CCSD:B97) | Δ(CCSD:ωB97X-V) | Δ(CCSD:ωB97M-V) |
| | NaO | $X^2\Pi$ | 526[b] | -31.86 | -30.77 | -29.95 | -30.34 | -30.32 | -30.43 | -30.74 | -30.43 |
| | MgH | $X^2\Sigma^+$ | 1492.7763[a] | 5.71 | 5.65 | 2.85 | 6.38 | 5.07 | 4.69 | 6.68 | 4.41 |
| | MgF | $X^2\Sigma^+$ | 711.69[b] | 8.65 | 10.70 | 11.32 | 11.61 | 11.24 | 11.14 | 10.76 | 10.96 |
| | $AlH^+$ | $X^2\Sigma^+$ | 1620[b] | 35.64 | 39.98 | 49.31 | 53.80 | 55.42 | 53.32 | 56.24 | 56.34 |

| | | | | | | | | | | | |
|---|---|---|---|---|---|---|---|---|---|---|---|
| | SiH | $X^2\Pi_r$ | 2042.5229[a] | 3.70 | 10.43 | 9.01 | 8.12 | 9.23 | 8.72 | 5.85 | 8.80 |
| | SiF | $X^2\Pi_r$ | 837.32507[a] | 25.35 | 29.11 | 30.25 | 31.16 | 29.92 | 29.82 | 29.22 | 29.28 |
| | PH | $X^3\Sigma^-$ | 2363.774[a] | 22.73 | 20.77 | 24.52 | 28.98 | 25.38 | 25.99 | 26.01 | 25.42 |
| | $PH^+$ | $X^2\Pi_r$ | 2299.6[b] | 111.17 | 106.73 | 108.42 | 110.46 | 110.30 | 111.31 | 109.79 | 111.25 |
| | $PH^-$ | $X^2\Pi_i$ | 2230[b] | 51.52 | 53.38 | 52.00 | 57.70 | 55.47 | 55.64 | 51.35 | 55.97 |
| | CP | $X^2\Sigma^+$ | 1239.79924[a] | 46.65 | 49.54 | 65.23 | 56.05 | 50.55 | 50.81 | 46.51 | 49.01 |
| | PO | $X^2\Pi_r$ | 1233.34[a] | 56.82 | 66.22 | 71.61 | 68.09 | 66.12 | 65.76 | 64.09 | 64.08 |
| | $PO^-$ | $X^3\Sigma^-$ | 1000[b] | 74.82 | 82.86 | 87.48 | 84.47 | 82.98 | 82.61 | 81.41 | 81.48 |
| | PF | $X^3\Sigma^-$ | 846.75[a] | 11.24 | 15.47 | 16.87 | 17.82 | 16.23 | 16.25 | 15.49 | 15.46 |
| | $PF^+$ | $X^2\Pi_r$ | 1053.25[b] | 22.32 | 31.21 | 33.88 | 34.16 | 32.02 | 31.73 | 30.52 | 30.60 |
| | HS | $X^2\Pi_i$ | 2696.2475[a] | 33.10 | 35.89 | 35.10 | 37.34 | 34.95 | 35.14 | 33.01 | 34.04 |
| | BS | $X^2\Sigma^+$ | 1179.91[a] | 31.87 | 35.92 | 39.48 | 39.23 | 37.17 | 37.24 | 34.95 | 35.84 |
| | $CS^+$ | $X^2\Sigma^+$ | 1384[b] | 50.49 | 60.63 | 72.80 | 65.99 | 59.11 | 60.42 | 56.66 | 58.66 |
| | NS | $X^2\Pi_r$ | 1218.7[b] | 51.77 | 68.59 | 78.28 | 69.90 | 66.09 | 65.95 | 62.92 | 63.65 |
| | SO | $X^3\Sigma^-$ | 1150.7913[a] | 50.36 | 59.71 | 64.42 | 59.59 | 57.70 | 57.53 | 56.15 | 56.34 |
| | $SO^+$ | $X^2\Pi_r$ | 1306.778[e] | 87.10 | 95.50 | 102.29 | 95.92 | 93.69 | 93.44 | 91.67 | 91.58 |
| | $HCl^+$ | $X^2\Pi_i$ | 2673.69[a] | 51.07 | 48.92 | 50.61 | 50.83 | 50.09 | 47.95 | 50.09 | 50.43 |
| | $LiCl^-$ | $X^2\Sigma^+$ | 480[b] | 29.43 | 29.89 | 29.55 | 30.19 | 29.52 | 29.54 | 29.86 | 29.65 |
| | BeCl | $X^2\Sigma^+$ | 846.7[b] | 1.99 | 2.41 | 2.76 | 3.28 | 2.99 | 2.83 | 2.48 | 2.63 |
| | CCl | $X^2\Pi$ | 876.89749[a] | 5.41 | 8.46 | 11.95 | 12.79 | 10.97 | 10.78 | 8.66 | 9.10 |
| | $ClF^+$ | $X^2\Pi$ | 870[b] | 82.04 | 101.77 | 109.34 | 106.86 | 102.63 | 102.89 | 100.22 | 100.43 |
| | NCl | $X^3\Sigma^-$ | 827.95767[a] | 0.17 | 1.02 | 5.88 | 7.27 | 4.12 | 4.14 | 1.93 | 1.87 |
| | OCl | $X^2\Pi_i$ | 853.64268[a] | 8.61 | 19.08 | 35.08 | 25.96 | 19.09 | 20.11 | 15.72 | 16.02 |
| | RMSD | | | 46.34 | 51.27 | 55.65 | 53.93 | 52.03 | 52.00 | 50.70 | 51.28 |
| | MSD | | | 34.37 | 39.23 | 43.35 | 42.36 | 40.29 | 40.20 | 38.80 | 39.36 |
| | MIN | | | -31.86 | -30.77 | -29.95 | -30.34 | -30.32 | -30.43 | -30.74 | -30.43 |
| | MAX | | | 111.17 | 106.73 | 109.34 | 110.46 | 110.30 | 111.31 | 109.79 | 111.25 |
| Row 3–Row 3 | Dimer | State | Expt. | Δ(CCSD: UHF) | Δ(CCSD: κ-OOMP2) | Δ(CCSD: OOMP2) | Δ(CCSD: BLYP) | Δ(CCSD: B97M-rV) | Δ(CCSD: B97) | Δ(CCSD: ωB97X-V) | Δ(CCSD: ωB97M-V) |
| | MgCl | $X^2\Sigma^+$ | 462.12[b] | 5.04 | 5.14 | 5.31 | 5.42 | 5.30 | 5.35 | 5.17 | 5.23 |
| | AlS | $X^2\Sigma^+$ | 617.1169[a] | -19.95 | -11.12 | -2.64 | -7.46 | -6.96 | -8.69 | -12.30 | -12.27 |
| | $Si_2$ | $X^3\Sigma_g^-$ | 510.98[a] | 20.68 | 21.66 | 55.58 | 23.52 | 22.94 | 22.99 | 21.82 | 21.99 |
| | SiCl | $X^2\Pi_r$ | 535.59[a] | -2.40 | -1.99 | -1.29 | -0.52 | -1.07 | -1.13 | -1.70 | -1.57 |
| | $P_2^+$ | $X^2\Pi_u$ | 672.2[a] | 49.78 | 49.27 | 106.91 | 51.80 | 50.71 | 50.83 | 49.06 | 49.28 |
| | PS | $X^2\Pi_r$ | 739.1[b] | 40.49 | 32.27 | 36.60 | 35.72 | 34.10 | 34.18 | 32.45 | 32.74 |
| | $S_2$ | $X^3\Sigma_g^-$ | 725.7102[a] | 22.26 | 24.59 | 26.94 | 26.26 | 25.43 | 25.24 | 24.32 | 24.48 |
| | $S_2^+$ | $X^2\Pi_{g,r}$ | 790[b] | 60.19 | 61.62 | 65.35 | 63.46 | 62.42 | 62.37 | 60.82 | 61.02 |
| | RMSD | | | 33.71 | 32.59 | 51.10 | 34.12 | 33.32 | 33.38 | 32.42 | 32.57 |
| | MSD | | | 22.01 | 22.68 | 36.59 | 24.78 | 24.11 | 23.89 | 22.46 | 22.61 |
| | MIN | | | -19.95 | -11.12 | -2.64 | -7.46 | -6.96 | -8.69 | -12.30 | -12.27 |

| | MAX | | | 60.19 | 61.62 | 106.91 | 63.46 | 62.42 | 62.37 | 60.82 | 61.02 |
|---|---|---|---|---|---|---|---|---|---|---|---|
| Open-shell | Dimer | State | Expt. | Δ(CCSD: UHF) | Δ(CCSD: $\kappa$-OOMP2) | Δ(CCSD: OOMP2) | Δ(CCSD: BLYP) | Δ(CCSD: B97M-rV) | Δ(CCSD: B97) | Δ(CCSD: $\omega$B97X-V) | Δ(CCSD: $\omega$B97M-V) |
| | RMSD | | | 56.78 | 61.44 | 66.86 | 62.65 | 60.23 | 60.17 | 58.60 | 59.06 |
| | MSD | | | 39.64 | 45.96 | 50.71 | 48.03 | 45.67 | 45.52 | 43.43 | 44.18 |
| | MIN | | | -65.13 | -49.85 | -47.22 | -49.21 | -50.23 | -50.31 | -50.52 | -50.67 |
| | MAX | | | 153.52 | 152.75 | 161.40 | 150.43 | 148.16 | 147.68 | 146.35 | 145.97 |

[a] From Ref. **?** .
[b] From Ref. **?** .
[d] From Ref. **?** .
[e] From Ref. **?** .
[*] Theoretical results.
